# Supplementary material for: Unity Forests: Improving Interaction Modelling and Interpretability in Random Forests
Source: arXiv:2601.07003 ancillary file (2026-01-11)
Supplement: Supplementary file 1 [file suppmat_unityforests.pdf]

Supplementary material to the article:

# **Unity Forests: Improving Interaction Modelling and Interpretability in Random Forests**

Roman Hornung<sup>\*,1,2</sup>

Alexander Hapfelmeier<sup>3,4</sup>

<sup>1</sup> Institute for Medical Information Processing, Biometry and Epidemiology, Faculty of Medicine, Ludwig Maximilian University of Munich (LMU), Marchioninistr. 15, Munich, 81377, Germany

<sup>2</sup> Munich Center for Machine Learning (MCML), Munich, Germany

<sup>3</sup> Institute of General Practice and Health Services Research, Department of Clinical Medicine, TUM School of Medicine and Health, Technical University of Munich (TUM), Orleansstr. 47, Munich, 81667, Germany

<sup>4</sup> Institute of AI and Informatics in Medicine, TUM School of Medicine and Health, Technical University of Munich (TUM), Munich, Germany

---

\*To whom correspondence should be addressed: [hornung@ibe.med.uni-muenchen.de](mailto:hornung@ibe.med.uni-muenchen.de)

# Contents

|          |                                                                                                                             |           |
|----------|-----------------------------------------------------------------------------------------------------------------------------|-----------|
| <b>A</b> | <b>Details on the UFO Framework</b>                                                                                         | <b>3</b>  |
| A.1      | Detailed Description of the UFO Algorithm for Tree Construction . . . . .                                                   | 3         |
| A.2      | Handling of Nominal Covariates in the UFO Framework . . . . .                                                               | 5         |
| A.3      | UFO Algorithm: Default Hyperparameters and Their Rationales . . . . .                                                       | 5         |
| A.4      | Unity VIM: Further Explanations, Default Hyperparameters, and Their Rationales                                              | 6         |
| <b>B</b> | <b>Further Information on the Large-Scale Real Data Evaluation</b>                                                          | <b>8</b>  |
| B.1      | Overview of the Datasets . . . . .                                                                                          | 8         |
| B.2      | Detailed Description of the Preliminary Study on the Appropriateness of Critical<br>Default Hyperparameter Values . . . . . | 13        |
| B.3      | Comparison of Dataset-Specific Performance Measure Values of UFOs and Conventional<br>RFs . . . . .                         | 16        |
| <b>C</b> | <b>Further Information on the Simulation Study</b>                                                                          | <b>17</b> |
| C.1      | Detailed Descriptions of the Covariate Effects Based on Simulated Datasets . . . .                                          | 17        |
| C.1.1    | DGP 1 . . . . .                                                                                                             | 17        |
| C.1.2    | DGP 2 . . . . .                                                                                                             | 18        |
| C.2      | Formal Descriptions of the DGPs . . . . .                                                                                   | 18        |
| C.2.1    | DGP 1 . . . . .                                                                                                             | 18        |
| C.2.2    | DGP 2 . . . . .                                                                                                             | 22        |
| C.3      | Mean AUC Values With 95% Confidence Intervals and Median Ranks With 25%<br>and 75% Quartiles . . . . .                      | 24        |
| C.3.1    | DGP 1 . . . . .                                                                                                             | 24        |
| C.3.2    | DGP 2 . . . . .                                                                                                             | 26        |
| <b>D</b> | <b>Additional Results from the Empirical Evaluation of the CRTR Algorithm</b>                                               | <b>30</b> |
| D.1      | Simulated Data: Unity VIM and Permutation VIM Values . . . . .                                                              | 30        |
| D.2      | Simulated Data: CRTRs for all Informative Covariates . . . . .                                                              | 31        |
| D.2.1    | DGP 1 . . . . .                                                                                                             | 31        |
| D.2.2    | DGP 2 . . . . .                                                                                                             | 40        |
| D.3      | Wine Dataset: Unity VIM and Permutation VIM Values . . . . .                                                                | 49        |

## A Details on the UFO Framework

### A.1 Detailed Description of the UFO Algorithm for Tree Construction

The following provides a detailed step-by-step description of the UFO algorithm:

1. *Sample observations for training.* Randomly draw a proportion `FRACT_N` of the  $n$  available observations. In all subsequent steps, only these subsampled observations are used and are referred to as the *tree sample*.
2. *Sample covariates for the tree root.* Randomly draw a proportion `PROP_VAR` of all covariates and denote the resulting set of covariates by  $\mathcal{S}$ .
3. *Grow candidate tree roots.* Grow `N_CAND_TREES` random tree roots of depth `MAX_DEPTH_ROOT` using only the covariates in  $\mathcal{S}$ :

For  $l = 1, \dots, \text{N\_CAND\_TREES}$ :

Define the first open node as the tree sample.

Repeat the following until no open nodes remain:

- a) Consider one of the open nodes and denote it by  $\mathcal{O}$ .
- b) Check the stop criteria:
  - Stop criterion 1:  $\mathcal{O}$  is at level `MAX_DEPTH_ROOT` of the tree.
  - Stop criterion 2:  $\mathcal{O}$  contains at most `N_MIN_ROOT` observations.
  - Stop criterion 3: None of the covariates in  $\mathcal{S}$  has at least two unique values in  $\mathcal{O}$ . If  $\mathcal{S}$  contains more than 500 covariates (which, for the default value of `PROP_VAR`, see Section 3.1.1 of the main paper, only occurs for high-dimensional data), a random subset of 500 covariates from  $\mathcal{S}$  is used to check for covariates with at least two unique values.
- c) If one of the stop criteria in b) is met, mark  $\mathcal{O}$  as a root leaf, remove it from the set of open nodes, and—if open nodes remain—continue with the next open node; otherwise, stop the procedure.
- d) Randomly draw the split covariate  $x_{spl}$  from the set of covariates with at least two unique values. If  $\mathcal{S}$  contains more than 500 covariates, use the same subset of 500 covariates considered when evaluating the stop criteria.
- e) Determine the  $n_{un}$  unique values of  $x_{spl}$  in  $\mathcal{O}$  and sort them as  $a_1, \dots, a_{n_{un}}$ .
- f) Compute the midpoints between the successive sorted values:  $c_m = (a_m + a_{m+1})/2$ , where  $m \in \{1, \dots, n_{un} - 1\}$ .
- g) Randomly select one of the  $c_m$  values as the split point  $c$ .
- h) Split  $\mathcal{O}$  into two child nodes,  $\mathcal{O}_L$  and  $\mathcal{O}_R$ , by assigning all observations in  $\mathcal{O}$  with  $x_{spl}$  values smaller than  $c$  to  $\mathcal{O}_L$  and all observations with  $x_{spl}$  values larger than  $c$  to  $\mathcal{O}_R$ .
- i) Add  $\mathcal{O}_L$  and  $\mathcal{O}_R$  to the set of open nodes.

4. *Select the best tree root.* Choose the tree root among the `N_CAND_TREES` candidates from the previous step that maximizes the *partition criterion*.

For classification, the partition criterion is defined as:

$$I = \sum_{m=1}^M \frac{N_m}{N} I_m, \quad (1)$$

$$\text{where } I = 1 - \sum_{k=1}^K p_k^2, \quad I_m = 1 - \sum_{k=1}^{K_m} p_{m,k}^2. \quad (2)$$

Here,  $N$  denotes the total number of observations in the tree sample, and  $M$  the number of root leaves in the respective candidate tree root. For each root leaf  $m \in \{1, \dots, M\}$ ,  $N_m$  denotes the number of observations in root leaf  $m$ . Furthermore,  $p_k$  is the proportion of observations belonging to class  $k$  in the tree sample, and  $p_{m,k}$  is the corresponding proportion within root leaf  $m$ . The total number of classes is  $K$ , and  $K_m$  is the number of classes present in root leaf  $m$ . Finally,  $I$  denotes the impurity of the full tree sample, and  $I_m$  the impurity within root leaf  $m$ .

For regression, the partition criterion is computed as:

$$V = \sum_{m=1}^M \frac{N_m}{N} V_m, \quad (3)$$

$$\text{where } V = \frac{1}{N} \sum_{i=1}^N (y_i - \bar{y})^2, \quad V_m = \frac{1}{N_m} \sum_{i=1}^{N_m} (y_{i,m} - \bar{y}_m)^2. \quad (4)$$

The notation for  $N$ ,  $M$ , and  $N_m$  is the same as in equations (1) and (2). Here,  $y_i$  denotes the outcome of observation  $i$  in the tree sample, and  $\bar{y}$  the corresponding sample mean. Similarly,  $y_{i,m}$  denotes the outcome of observation  $i$  in root leaf  $m$ , and  $\bar{y}_m$  the mean outcome in root leaf  $m$ . Accordingly,  $V$  is the empirical variance of the outcome in the tree sample, and  $V_m$  the empirical variance within root leaf  $m$ .

5. *Expand the tree root using conventional splitting.* Expand each selected tree root into a full tree using the standard recursive splitting procedure of CART trees in random forests. For each split, a random subset of MTRY candidate covariates from all covariates is considered. Recursive splitting is stopped for nodes that satisfy one of the stop criteria from step 3 b), where corresponding parameters `MAX_DEPTH` and `N_MIN` are used. Stop criterion 3 is slightly modified here: it is met when none of the MTRY sampled candidate covariates has at least two unique values (rather than using random subsets of MTRY covariates for `MTRY > 500`).

The partition criterion increases as the tree leaves become purer with respect to class membership (for classification) or as the within-leaf variance decreases (for regression). This criterion thus represents a multi-way analogue of the Gini impurity reduction or variance reduction used in conventional binary splitting in CART trees.

## A.2 Handling of Nominal Covariates in the UFO Framework

As described in Section 3.1.2 of the main paper, the tree construction procedure of the UFO framework does not directly apply to nominal covariates. Therefore, the categories of such covariates are ordered using the procedure `respect.unordered.factors = "order"` implemented in the R package **ranger** (version 0.17.0).

For categorical outcomes with two classes, the categories are ordered according to the proportion of observations in each category that belong to the second class. For categorical outcomes with more than two classes, the procedure of Coppersmith et al. (1999) is applied. Specifically, for each nominal covariate, the relative frequencies of observations from each outcome class are computed for all  $J$  categories, resulting in a  $J \times C$  matrix, where  $C$  denotes the number of outcome classes. A weighted principal component analysis (PCA) is then performed on this matrix, using the category frequencies as weights. The ordering of categories is derived from the scores on the first principal component, ensuring that categories with similar outcome distributions are positioned close to each other.

For continuous outcomes, the categories are ordered according to the mean outcome values of the observations falling into each category.

## A.3 UFO Algorithm: Default Hyperparameters and Their Rationales

In the following, we describe and justify the chosen default values in the UFO algorithm.

Many of the UFO algorithm’s hyperparameters are shared with conventional RFs. For the parameters `MTRY`, `MAX_DEPTH`, and `N_MIN`, we adopt the default values from the R package **ranger**, on which the R package **unityForest**—in which UFOs are implemented—is largely based, with one exception noted below. Specifically, the default value for `MTRY` is  $\lfloor \sqrt{p} \rfloor$ , where  $p$  denotes the number of covariates. For `MAX_DEPTH`, the default value is  $\infty$ , corresponding to no restriction on tree depth. For `N_MIN`, the default value is 1 for classification, 5 for regression, and 5 for probability prediction. The latter differs from **ranger**, where the default for `N_MIN` in probability estimation is 10. We reduce this to 5 to allow deeper trees for small datasets, since deeper trees in RFs typically reduce both tree bias and inter-tree correlation. These RF-related hyperparameters serve the same purposes as in conventional RFs, and there is no reason to assume that alternative defaults would be more suitable in the context of the UFO algorithm.

Instead of using bootstrapping to draw the training samples for the trees, as is classically performed in RFs, we subsample a proportion of `FRACT_N = 0.7` for each tree. This choice follows the results of the real-data analysis reported in Probst et al. (2019). The number of constructed trees, `N_TREES`, is set to 20,000. This high number is motivated by the algorithm used for computing the unity VIM, as explained in the next subsection.

As described in Section 3.1.1 of the main paper, the proportion of drawn covariates `PROP_VAR` for each tree root is by default set to  $\sqrt{p}/p$  for  $p \leq 100$  and to 0.1 for  $p > 100$ . As with `N_TREES`, this choice is motivated by considerations related to the unity VIM calculation and is discussed in detail in the next subsection.

When the number of drawn covariates exceeds 500, only a random subset of 500 covariates is evaluated for stop criterion 3 in the UFO algorithm. This restriction prevents computational inefficiency for ultra-high-dimensional data, since the number `PROP_VAR · p` can become large when

`PROP_VAR` = 0.1 (the default value). For example, if  $p = 100,000$ , the number of drawn covariates is 10,000, making it computationally expensive to check all 10,000 covariates for at least two unique values in the respective nodes before sampling each split point during candidate tree root generation. Nonetheless, as discussed in Section 7 of the main paper, the UFO framework has inherent limitations for high-dimensional data settings.

For `N_CAND_TREES`, we set a default of 500. This represents a sufficiently large number of randomly generated candidate tree roots per tree root (see Section B.2 of this supplementary material and Section 6 of the main paper), while maintaining a reasonable computational cost. Increasing this number would yield tree roots closer to the optimal partition, but—as discussed in Section 3.1.1 of the main paper—this is neither necessary nor desirable, as it would likely increase correlation among tree predictions.

The default depth of tree roots, `MAX_DEPTH_ROOT`, is set to 3. Tree roots of depth three can capture marginal effects as well as two-way and three-way interactions. Higher-order interactions are likely rare in practice and, even when present, are difficult to interpret. Furthermore, the number of possible interacting covariate tuples increases rapidly with interaction order,<sup>1</sup> which reduces the statistical power to distinguish genuine interaction effects from random noise. Moreover, deeper trees may not reliably reproduce higher-order interactions, as numerous deep tree roots may produce partitions of the covariate space that are nearly equivalent to the optimal one.

The final hyperparameter is `N_MIN_ROOT`, which specifies the minimum number of observations in a node of the tree roots required for further splitting during candidate tree root generation. We set this value to 10 to prevent nodes from fragmenting into overly small subnodes. Since the tree roots are used both in the computation of the unity VIM (Section 3.2 of the main paper) and in determining the CRTRs for interpreting covariate effects (Section 3.3 of the main paper), it is essential that they capture data patterns that are reasonably stable and supported by an adequate number of observations. This restriction on node size, imposed by `N_MIN_ROOT` = 10, is particularly relevant for small datasets, where overly small nodes would otherwise be more likely to occur.

#### A.4 Unity VIM: Further Explanations, Default Hyperparameters, and Their Rationales

The use of the reduction in Gini impurity or variance in the unity VIM algorithm is consistent with the long-popular mean decrease in impurity (MDI). However, by computing these quantities on the OOB data, the unity VIM avoids the biases known to affect the MDI, following Li et al. (2019), Loecher (2020), and Zhou and Hooker (2021).

Subtracting the reduction in Gini impurity or variance obtained after permuting the covariate values ensures that the unity VIM values for non-informative covariates fluctuate symmetrically around zero. One might expect that the reductions in Gini impurity or variance calculated on the OOB data would already be centered around zero for non-informative covariates, even without this subtraction. However, random splits in non-informative covariates can still lead to small reductions in Gini impurity or variance, which would otherwise induce a slight positive bias in the unity VIM values (results not shown).

---

<sup>1</sup>In a dataset with  $p$  covariates, there are  $\binom{p}{k}$  possible  $k$ -way interactions.

As described earlier, the following default values are used for the proportion of covariates considered for each tree root, `PROP_VAR`:  $\sqrt{p}/p$  for  $p \leq 100$  and 0.1 for  $p > 100$ , where  $p$  denotes the number of covariates. Considering only a relatively small subset of covariates per tree root prevents the same strongly influential covariates from dominating across all tree roots. Consequently, interaction effects without marginal effects will be represented each in sufficiently large proportions of trees. The default values for `PROP_VAR` ensure that the proportion of covariates considered per tree root is not less than 0.1. Ignoring, for simplicity, that covariates are drawn without replacement, the probability that both members of an interacting covariate pair are included in the same tree root is approximately 0.01 ( $0.1 \cdot 0.1$ ). Hence, the corresponding interaction effect can be expected to be reflected in 1% of the trees. This reasoning motivates the default value `PROP_BEST_SPLITS` = 0.01 for the proportion of top-scoring splits selected per covariate.

Because `PROP_BEST_SPLITS` is small, a large number of trees is required to ensure that enough highly informative splits are available for the unity VIM calculation. For this reason, the default number of trees is set to `N_TREES` = 20,000. Because only every hundredth split in a covariate contributes to the unity VIM, this setting corresponds approximately to using 200 trees ( $20,000 \times 0.01$ ) in a setting where every split were considered. These two scenarios are not perfectly comparable, however: focusing on the top 1% of splits for informative covariates prioritizes particularly discriminative splits, whereas including all splits introduces greater heterogeneity in discriminative strength and, consequently, higher variability.

When using the default value `N_TREES` = 20,000, the situation in which the number of top 1% splits (corresponding to `PROP_BEST_SPLITS` = 0.01) would fall below five—thus triggering the fallback to using five or fewer best splits—did not occur in either the simulation study or the real-data analyses. Instead, the resulting numbers of top splits were consistently much higher (results not shown), suggesting that the default of 20,000 trees is sufficiently large.

## B Further Information on the Large-Scale Real Data Evaluation

### B.1 Overview of the Datasets

Table S1: Overview of datasets – I. The following information is provided: ‘data.id’: OpenML ID of the dataset, ‘label’: dataset label, ‘n’: sample size, ‘p’: number of covariates, ‘prop. categ.’: proportion of categorical covariates, ‘prop. min. class’: proportion of observations in the smaller class of the target variable, ‘study’: indicator whether the dataset was used in the preliminary analysis (‘pre’) or the comparison study (‘main’)

| data.id | label                       | n     | p   | prop. categ. | prop. min. class | study |
|---------|-----------------------------|-------|-----|--------------|------------------|-------|
| 31      | credit-g                    | 1000  | 20  | 0.650        | 0.300            | main  |
| 37      | diabetes                    | 768   | 8   | 0.000        | 0.349            | main  |
| 40      | sonar                       | 208   | 60  | 0.000        | 0.466            | main  |
| 43      | haberman                    | 306   | 3   | 0.000        | 0.265            | main  |
| 44      | spambase                    | 4601  | 57  | 0.000        | 0.394            | main  |
| 50      | tic-tac-toe                 | 958   | 9   | 1.000        | 0.347            | main  |
| 53      | heart-statlog               | 270   | 13  | 0.385        | 0.444            | main  |
| 59      | ionosphere                  | 351   | 33  | 0.000        | 0.359            | main  |
| 164     | molecular-biology_promoters | 106   | 57  | 1.000        | 0.500            | main  |
| 292     | Australian                  | 690   | 14  | 0.000        | 0.445            | main  |
| 310     | mammography                 | 10000 | 6   | 0.000        | 0.023            | main  |
| 311     | oil_spill                   | 937   | 48  | 0.000        | 0.044            | main  |
| 312     | scene                       | 2407  | 299 | 0.017        | 0.179            | main  |
| 316     | yeast_ml8                   | 2417  | 116 | 0.112        | 0.014            | main  |
| 333     | monks-problems-1            | 556   | 6   | 1.000        | 0.500            | main  |
| 337     | SPECTF                      | 349   | 44  | 0.000        | 0.272            | main  |
| 346     | aids                        | 50    | 4   | 0.500        | 0.500            | main  |
| 350     | webdata_wXa                 | 10000 | 121 | 0.000        | 0.238            | main  |
| 357     | vehicle_sensIT              | 10000 | 100 | 0.000        | 0.492            | main  |
| 444     | analcata_data_boxing2       | 132   | 3   | 1.000        | 0.462            | main  |
| 446     | prnn_crabs                  | 200   | 7   | 0.143        | 0.500            | main  |
| 450     | analcata_data_lawsuit       | 264   | 4   | 0.250        | 0.072            | main  |
| 459     | analcata_data_asbestos      | 83    | 3   | 0.667        | 0.446            | main  |
| 467     | analcata_data_japansolvent  | 52    | 8   | 0.000        | 0.481            | main  |
| 472     | lupus                       | 87    | 3   | 0.000        | 0.402            | main  |
| 476     | analcata_data_bankruptcy    | 50    | 5   | 0.000        | 0.500            | main  |
| 479     | analcata_data_cyyoung9302   | 92    | 9   | 0.333        | 0.207            | main  |
| 682     | sleuth_ex2016               | 87    | 10  | 0.100        | 0.414            | main  |
| 683     | sleuth_ex2015               | 60    | 7   | 0.000        | 0.500            | main  |
| 714     | fruitfly                    | 125   | 4   | 0.500        | 0.392            | main  |
| 717     | rmftsa_ladata               | 508   | 10  | 0.000        | 0.437            | pre   |
| 719     | veteran                     | 137   | 7   | 0.571        | 0.314            | pre   |
| 720     | abalone                     | 4177  | 8   | 0.125        | 0.498            | main  |
| 721     | pwLinear                    | 200   | 10  | 0.000        | 0.485            | pre   |
| 722     | pol                         | 10000 | 26  | 0.000        | 0.333            | main  |
| 724     | analcata_data_vineyard      | 468   | 3   | 0.000        | 0.444            | main  |
| 725     | bank8FM                     | 8192  | 8   | 0.000        | 0.404            | main  |
| 728     | analcata_data_supreme       | 4052  | 7   | 0.000        | 0.240            | pre   |
| 729     | visualizing_slope           | 44    | 3   | 0.000        | 0.386            | main  |

Table S2: Overview of datasets – II. The following information is provided: ‘data.id’: OpenML ID of the dataset, ‘label’: dataset label, ‘n’: sample size, ‘p’: number of covariates, ‘prop. categ.’: proportion of categorical covariates, ‘prop. min. class’: proportion of observations in the smaller class of the target variable, ‘study’: indicator whether the dataset was used in the preliminary analysis (‘pre’) or the comparison study (‘main’)

| data.id | label                     | n     | p  | prop. categ. | prop. min. class | study |
|---------|---------------------------|-------|----|--------------|------------------|-------|
| 731     | basketball                | 96    | 4  | 0.000        | 0.490            | main  |
| 733     | machine_cpu               | 209   | 6  | 0.000        | 0.268            | pre   |
| 734     | aileron                   | 10000 | 40 | 0.000        | 0.424            | pre   |
| 736     | visualizing_environmental | 111   | 3  | 0.000        | 0.477            | main  |
| 737     | space_ga                  | 3107  | 6  | 0.000        | 0.496            | pre   |
| 741     | rmftsa_sleepdata          | 1024  | 2  | 0.500        | 0.497            | main  |
| 745     | auto_price                | 159   | 15 | 0.067        | 0.340            | main  |
| 747     | servo                     | 167   | 4  | 1.000        | 0.228            | main  |
| 748     | analcata_wildcat          | 163   | 5  | 0.400        | 0.288            | pre   |
| 750     | pm10                      | 500   | 7  | 0.000        | 0.492            | main  |
| 753     | wisconsin                 | 194   | 32 | 0.000        | 0.464            | pre   |
| 755     | sleuth_ex1605             | 62    | 5  | 0.000        | 0.500            | main  |
| 758     | analcata_election2000     | 67    | 14 | 0.000        | 0.269            | main  |
| 759     | analcata_olympic2000      | 66    | 11 | 0.000        | 0.500            | main  |
| 761     | cpu_act                   | 8192  | 21 | 0.000        | 0.302            | main  |
| 767     | analcata_apnea1           | 475   | 3  | 0.667        | 0.128            | main  |
| 770     | strikes                   | 625   | 6  | 0.000        | 0.496            | pre   |
| 771     | analcata_michiganacc      | 108   | 3  | 0.667        | 0.444            | pre   |
| 772     | quake                     | 2178  | 3  | 0.000        | 0.445            | main  |
| 774     | disclosure_x_bias         | 662   | 3  | 0.000        | 0.479            | main  |
| 777     | sleuth_ex1714             | 47    | 7  | 0.000        | 0.426            | main  |
| 778     | bodyfat                   | 252   | 14 | 0.000        | 0.492            | main  |
| 780     | rabe_265                  | 51    | 6  | 0.000        | 0.412            | main  |
| 782     | rabe_266                  | 120   | 2  | 0.000        | 0.475            | pre   |
| 784     | newton_hema               | 140   | 3  | 0.333        | 0.500            | main  |
| 787     | witmer_census_1980        | 50    | 4  | 0.000        | 0.480            | main  |
| 788     | triazines                 | 186   | 58 | 0.000        | 0.414            | main  |
| 790     | elusage                   | 55    | 2  | 0.500        | 0.436            | pre   |
| 791     | diabetes_numeric          | 43    | 2  | 0.000        | 0.395            | main  |
| 800     | pyrim                     | 74    | 26 | 0.000        | 0.419            | main  |
| 801     | chscase_funds             | 185   | 2  | 0.000        | 0.470            | main  |
| 803     | delta_aileron             | 7129  | 5  | 0.000        | 0.469            | pre   |
| 804     | hutsof99_logis            | 70    | 7  | 0.571        | 0.486            | main  |
| 807     | kin8nm                    | 8192  | 8  | 0.000        | 0.491            | main  |
| 811     | rmftsa_ctoarrivals        | 264   | 2  | 0.500        | 0.383            | main  |
| 814     | chscase_vine2             | 468   | 2  | 0.000        | 0.453            | pre   |
| 815     | chscase_vine1             | 52    | 8  | 0.000        | 0.462            | main  |
| 816     | puma8NH                   | 8192  | 8  | 0.000        | 0.498            | pre   |
| 817     | digggle_table_a1          | 48    | 3  | 0.000        | 0.479            | pre   |
| 818     | digggle_table_a2          | 310   | 8  | 0.125        | 0.468            | pre   |
| 819     | delta_elevators           | 9517  | 6  | 0.000        | 0.497            | main  |
| 820     | chatfield_4               | 235   | 12 | 0.000        | 0.396            | pre   |
| 821     | house_16H                 | 10000 | 16 | 0.000        | 0.292            | main  |
| 823     | houses                    | 10000 | 8  | 0.000        | 0.434            | pre   |
| 826     | sensory                   | 576   | 11 | 1.000        | 0.415            | pre   |

Table S3: Overview of datasets – III. The following information is provided: ‘data.id’: OpenML ID of the dataset, ‘label’: dataset label, ‘n’: sample size, ‘p’: number of covariates, ‘prop. categ.’: proportion of categorical covariates, ‘prop. min. class’: proportion of observations in the smaller class of the target variable, ‘study’: indicator whether the dataset was used in the preliminary analysis (‘pre’) or the comparison study (‘main’)

| data.id | label                  | n     | p   | prop. categ. | prop. min. class | study |
|---------|------------------------|-------|-----|--------------|------------------|-------|
| 835     | analcata_vehicle       | 48    | 4   | 0.750        | 0.438            | main  |
| 841     | stock                  | 950   | 9   | 0.000        | 0.486            | main  |
| 846     | elevators              | 10000 | 18  | 0.000        | 0.306            | main  |
| 847     | wind                   | 6574  | 14  | 0.000        | 0.467            | main  |
| 848     | schlvote               | 38    | 5   | 0.200        | 0.263            | main  |
| 851     | tecator                | 240   | 124 | 0.000        | 0.425            | pre   |
| 853     | boston                 | 506   | 13  | 0.077        | 0.413            | pre   |
| 857     | bolts                  | 40    | 7   | 0.000        | 0.350            | pre   |
| 859     | analcata_gviolence     | 74    | 8   | 0.000        | 0.419            | main  |
| 860     | vinnie                 | 380   | 2   | 0.000        | 0.487            | main  |
| 874     | rabe_131               | 50    | 4   | 0.000        | 0.420            | main  |
| 875     | analcata_chlamydia     | 100   | 3   | 0.667        | 0.190            | main  |
| 880     | mu284                  | 284   | 9   | 0.000        | 0.500            | main  |
| 882     | pollution              | 60    | 15  | 0.000        | 0.483            | main  |
| 885     | transplant             | 131   | 2   | 0.000        | 0.366            | main  |
| 886     | no2                    | 500   | 7   | 0.000        | 0.498            | pre   |
| 887     | mbagrade               | 61    | 2   | 0.500        | 0.475            | main  |
| 890     | cloud                  | 108   | 7   | 0.143        | 0.296            | main  |
| 892     | sleuth_case1201        | 50    | 6   | 0.000        | 0.480            | main  |
| 893     | visualizing_hamster    | 73    | 5   | 0.000        | 0.452            | main  |
| 894     | rabe_148               | 66    | 5   | 0.000        | 0.500            | main  |
| 895     | chscase_geyser1        | 222   | 2   | 0.000        | 0.396            | pre   |
| 902     | sleuth_case2002        | 147   | 6   | 0.667        | 0.469            | main  |
| 905     | chscase_adopt          | 39    | 2   | 0.000        | 0.308            | main  |
| 906     | chscase_census5        | 400   | 7   | 0.000        | 0.482            | main  |
| 914     | balloon                | 2001  | 1   | 0.000        | 0.241            | main  |
| 915     | plasma_retinol         | 315   | 13  | 0.231        | 0.422            | main  |
| 919     | rabe_166               | 40    | 1   | 0.000        | 0.475            | pre   |
| 921     | analcata_seropositive  | 132   | 3   | 0.333        | 0.348            | pre   |
| 923     | visualizing_soil       | 8641  | 4   | 0.250        | 0.450            | main  |
| 924     | humandevol             | 130   | 1   | 0.000        | 0.500            | main  |
| 925     | visualizing_galaxy     | 323   | 4   | 0.000        | 0.458            | main  |
| 927     | hutsof99_child_witness | 42    | 15  | 0.000        | 0.405            | pre   |
| 929     | rabe_176               | 70    | 3   | 0.000        | 0.500            | main  |
| 934     | socmob                 | 1156  | 5   | 0.800        | 0.221            | main  |
| 945     | kidney                 | 76    | 5   | 0.600        | 0.474            | main  |
| 946     | visualizing_ethanol    | 88    | 2   | 0.000        | 0.489            | main  |
| 949     | arsenic-female-bladder | 559   | 3   | 0.000        | 0.143            | pre   |
| 954     | spectrometer           | 531   | 100 | 0.010        | 0.104            | main  |
| 955     | tae                    | 151   | 5   | 0.800        | 0.344            | main  |
| 958     | segment                | 2310  | 18  | 0.000        | 0.143            | main  |
| 959     | nursery                | 10000 | 8   | 1.000        | 0.332            | main  |
| 962     | mfeat-morphological    | 2000  | 6   | 0.000        | 0.100            | main  |
| 964     | pasture                | 36    | 21  | 0.048        | 0.333            | main  |
| 965     | zoo                    | 101   | 16  | 0.938        | 0.406            | main  |

Table S4: Overview of datasets – IV. The following information is provided: ‘data.id’: OpenML ID of the dataset, ‘label’: dataset label, ‘n’: sample size, ‘p’: number of covariates, ‘prop. categ.’: proportion of categorical covariates, ‘prop. min. class’: proportion of observations in the smaller class of the target variable, ‘study’: indicator whether the dataset was used in the preliminary analysis (‘pre’) or the comparison study (‘main’)

| data.id | label                   | n     | p    | prop. categ. | prop. min. class | study |
|---------|-------------------------|-------|------|--------------|------------------|-------|
| 969     | iris                    | 150   | 4    | 0.000        | 0.333            | main  |
| 970     | analcadata_authorship   | 841   | 70   | 0.000        | 0.377            | main  |
| 971     | mfeat-fourier           | 2000  | 76   | 0.000        | 0.100            | main  |
| 973     | wine                    | 178   | 13   | 0.000        | 0.399            | main  |
| 974     | hayes-roth              | 132   | 4    | 0.750        | 0.386            | main  |
| 976     | JapaneseVowels          | 9961  | 14   | 0.000        | 0.162            | main  |
| 977     | letter                  | 10000 | 16   | 0.000        | 0.040            | main  |
| 978     | mfeat-factors           | 2000  | 216  | 0.000        | 0.100            | main  |
| 980     | optdigits               | 5620  | 62   | 0.000        | 0.102            | main  |
| 983     | cmc                     | 1473  | 9    | 0.778        | 0.427            | main  |
| 987     | collins                 | 500   | 21   | 0.048        | 0.160            | main  |
| 988     | fl2000                  | 67    | 15   | 0.067        | 0.388            | main  |
| 991     | car                     | 1728  | 6    | 1.000        | 0.300            | main  |
| 994     | vehicle                 | 846   | 18   | 0.000        | 0.258            | main  |
| 995     | mfeat-zernike           | 2000  | 47   | 0.000        | 0.100            | main  |
| 997     | balance-scale           | 625   | 4    | 0.000        | 0.461            | main  |
| 1005    | glass                   | 214   | 9    | 0.000        | 0.355            | main  |
| 1009    | white-clover            | 63    | 31   | 0.129        | 0.397            | main  |
| 1011    | ecoli                   | 336   | 7    | 0.000        | 0.426            | main  |
| 1013    | analcadata_challenger   | 138   | 2    | 0.500        | 0.065            | main  |
| 1014    | analcadata_dmft         | 797   | 4    | 1.000        | 0.194            | main  |
| 1015    | confidence              | 72    | 3    | 0.000        | 0.167            | main  |
| 1016    | vowel                   | 990   | 13   | 0.231        | 0.091            | main  |
| 1019    | pendigits               | 10000 | 16   | 0.000        | 0.104            | main  |
| 1020    | mfeat-karhunen          | 2000  | 64   | 0.000        | 0.100            | main  |
| 1021    | page-blocks             | 5473  | 10   | 0.000        | 0.102            | main  |
| 1022    | mfeat-pixel             | 2000  | 240  | 1.000        | 0.100            | main  |
| 1025    | analcadata_germangss    | 400   | 5    | 1.000        | 0.225            | main  |
| 1036    | sylva_agnostic          | 10000 | 212  | 0.000        | 0.060            | main  |
| 1038    | gina_agnostic           | 3468  | 970  | 0.000        | 0.492            | main  |
| 1039    | hiva_agnostic           | 4229  | 1000 | 1.000        | 0.035            | main  |
| 1043    | ada_agnostic            | 4562  | 47   | 0.000        | 0.248            | main  |
| 1046    | mozilla4                | 10000 | 4    | 0.250        | 0.327            | main  |
| 1048    | jEdit_4.2.4.3           | 369   | 8    | 0.000        | 0.447            | main  |
| 1054    | mc2                     | 161   | 39   | 0.000        | 0.323            | main  |
| 1061    | ar4                     | 107   | 29   | 0.000        | 0.187            | main  |
| 1067    | kc1                     | 2109  | 21   | 0.000        | 0.155            | main  |
| 1073    | jEdit_4.0.4.2           | 274   | 8    | 0.000        | 0.489            | main  |
| 1121    | badges2                 | 294   | 10   | 0.300        | 0.286            | main  |
| 1176    | Internet-Advertisements | 3279  | 1000 | 0.000        | 0.140            | main  |
| 1441    | KungChi3                | 123   | 39   | 0.000        | 0.130            | main  |
| 1442    | MegaWatt1               | 253   | 37   | 0.000        | 0.107            | main  |
| 1444    | PizzaCutter3            | 1043  | 37   | 0.000        | 0.122            | main  |
| 1447    | CastMetal1              | 327   | 37   | 0.000        | 0.128            | main  |
| 1454    | PieChart4               | 1458  | 37   | 0.000        | 0.122            | main  |

Table S5: Overview of datasets – V. The following information is provided: ‘data.id’: OpenML ID of the dataset, ‘label’: dataset label, ‘n’: sample size, ‘p’: number of covariates, ‘prop. categ.’: proportion of categorical covariates, ‘prop. min. class’: proportion of observations in the smaller class of the target variable, ‘study’: indicator whether the dataset was used in the preliminary analysis (‘pre’) or the comparison study (‘main’)

| data.id | label                            | n     | p   | prop. categ. | prop. min. class | study |
|---------|----------------------------------|-------|-----|--------------|------------------|-------|
| 1455    | acute-inflammations              | 120   | 6   | 0.833        | 0.417            | main  |
| 1461    | bank-marketing                   | 10000 | 16  | 0.562        | 0.126            | main  |
| 1462    | banknote-authentication          | 1372  | 4   | 0.000        | 0.445            | main  |
| 1463    | blogger                          | 100   | 5   | 1.000        | 0.320            | main  |
| 1464    | blood-transfusion-service-center | 748   | 4   | 0.000        | 0.238            | main  |
| 1467    | climate-model-simulation-crashes | 540   | 20  | 0.000        | 0.085            | main  |
| 1471    | eeg-eye-state                    | 10000 | 14  | 0.000        | 0.449            | main  |
| 1473    | fertility                        | 100   | 9   | 0.000        | 0.120            | main  |
| 1479    | hill-valley                      | 1212  | 100 | 0.000        | 0.500            | main  |
| 1480    | ilpd                             | 583   | 10  | 0.100        | 0.286            | main  |
| 1487    | ozone-level-8hr                  | 2534  | 72  | 0.000        | 0.063            | main  |
| 1488    | parkinsons                       | 195   | 22  | 0.000        | 0.246            | main  |
| 1489    | phoneme                          | 5404  | 5   | 0.000        | 0.293            | main  |
| 1490    | planning-relax                   | 182   | 12  | 0.000        | 0.286            | main  |
| 1494    | qsar-biodeg                      | 1055  | 41  | 0.000        | 0.337            | main  |
| 1495    | qualitative-bankruptcy           | 250   | 6   | 1.000        | 0.428            | main  |
| 1498    | sa-heart                         | 462   | 9   | 0.111        | 0.346            | main  |
| 1502    | skin-segmentation                | 10000 | 3   | 0.000        | 0.212            | main  |
| 1504    | steel-plates-fault               | 1941  | 33  | 0.000        | 0.347            | main  |
| 1510    | wdbc                             | 569   | 30  | 0.000        | 0.373            | main  |
| 1511    | wholesale-customers              | 440   | 8   | 0.125        | 0.323            | main  |
| 1524    | vertebra-column                  | 310   | 6   | 0.000        | 0.323            | main  |
| 1547    | autoUniv-au1-1000                | 1000  | 20  | 1.000        | 0.259            | main  |
| 1570    | wilt                             | 4839  | 5   | 0.000        | 0.054            | main  |

## B.2 Detailed Description of the Preliminary Study on the Appropriateness of Critical Default Hyperparameter Values

Of the 198 available datasets, 92 were obtained by dichotomizing a continuous outcome, according to the dataset descriptions on OpenML. Although dichotomization of continuous outcomes is common in practice—since the main interest often lies in whether a value exceeds a certain threshold—datasets with inherently binary outcomes typically exhibit clearer class separation. In contrast, for dichotomized outcomes, observations become increasingly similar as their underlying continuous values approach the cutoff between classes.

Because the number of available datasets was large but finite, and to retain more datasets with inherently binary outcomes for the large-scale comparison between UFOs and conventional RFs, we randomly selected the 30 datasets used in this preliminary study from the subset of 92 datasets with dichotomized outcomes. Tables S1–S5 of this supplementary material indicate which of the 198 datasets were used in the preliminary study.

Each of the three considered hyperparameters was varied separately across a grid of meaningful values—including the default value—and the predictive performance of UFOs was evaluated on the 30 selected datasets. The goal was twofold: (i) to examine whether the chosen default values yield predictive performance close to the optimum among all considered values, and (ii) to assess how sensitive predictive performance is to changes in each hyperparameter. While varying one hyperparameter, all others were fixed at their default values as specified in Sections A.3 and A.4 of this supplementary material.

The only exception was the number of constructed trees, `N_TREES`, which we set to 2,000 instead of 20,000. This reduction was necessary because some grid configurations were computationally demanding, and using fewer trees substantially reduced the computation time. The high default value of 20,000 is motivated by the unity VIM algorithm (see Section 3.2 of the main paper), but it is unlikely that the predictive performance of UFOs increases meaningfully for `N_TREES` values above 2,000.

Predictive performance was assessed for each combination of hyperparameter value and dataset using five-fold stratified cross-validation repeated five times. The Brier score (**Brier**), the area under the ROC curve (**AUC**), and the accuracy (**ACC**) were used as performance measures.

The number of random candidate trees, `N_CAND_TREES`, determines how closely the selected tree roots approximate the optimal tree roots that could be obtained given the covariates considered for each root. A closer approximation can lead to purer partitions but may also increase the correlation among the tree roots, potentially reducing the forest’s predictive performance. We considered the following grid for `N_CAND_TREES`: 2, 5, 10, 50, 100, 200, 500, 1,000, 2,000.

Figure S1 presents the results for the three hyperparameters. For nearly all datasets, `N_CAND_TREES` had little or no notable influence on predictive performance. For one dataset, a minor deterioration in **Brier** was observed at higher values. In contrast, small improvements in **ACC** appeared for larger `N_CAND_TREES` values in some datasets, with a more pronounced effect in one case. Beyond the chosen default value of `N_CAND_TREES` = 500, however, no further improvements in accuracy were observed for any dataset, suggesting that this default value is appropriate.

The depth of the tree roots, `MAX_DEPTH_ROOT`, determines the maximum order of interactions that can be represented. As described in Section A.3, the default value is set to 3, allowing the

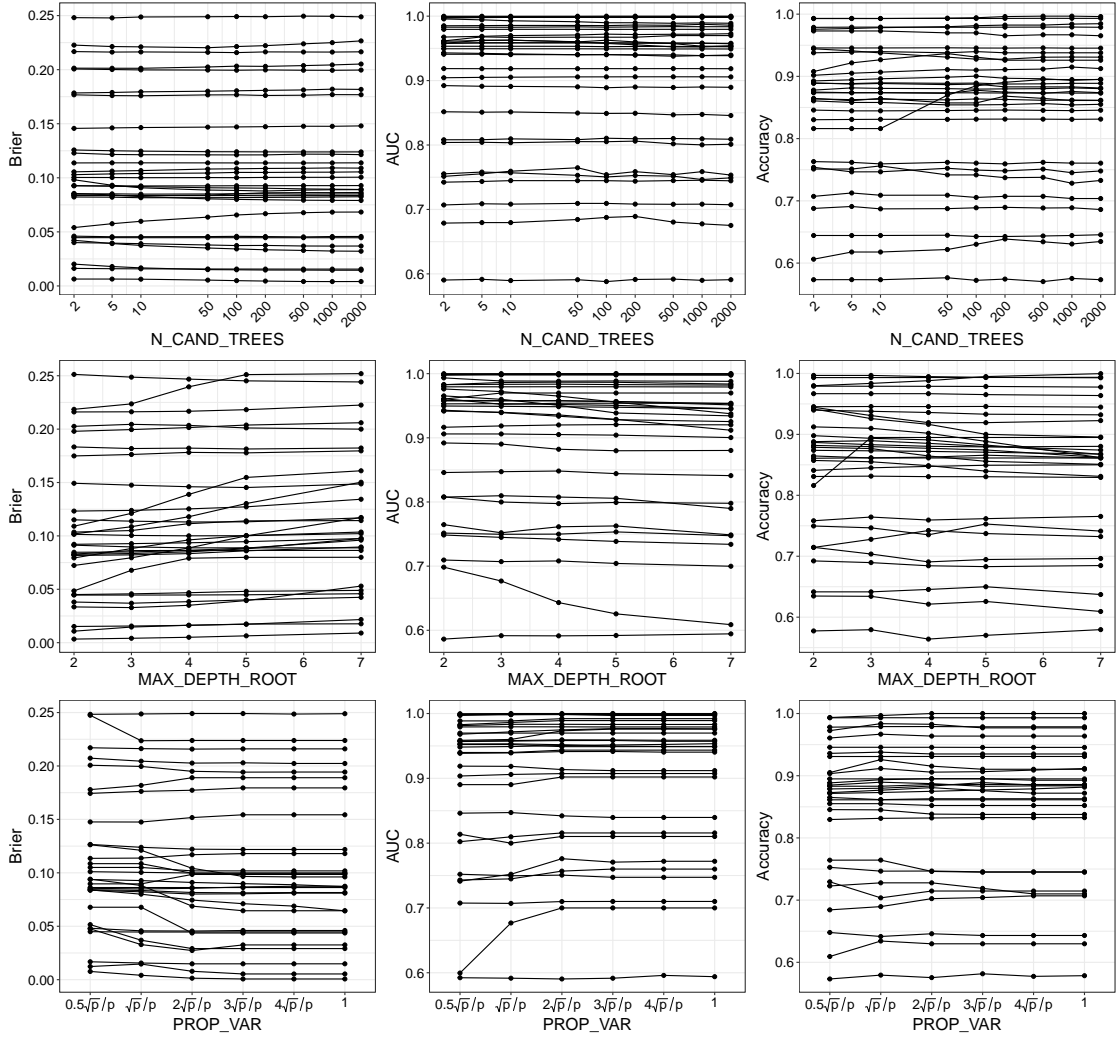

Fig. S1: Preliminary study: Dataset-specific performance metric values depending on the considered values of N\_CAND\_TREES, MAX\_DEPTH\_ROOT, and PROP\_VAR

tree roots to model up to three-way interactions. This choice was made primarily for reasons of interpretability (see Section A.3). However, it was not clear whether alternative values of MAX\_DEPTH\_ROOT might yield better predictive performance.

We therefore evaluated the grid 2, 3, 4, 5, 7. Similar to the results for N\_CAND\_TREES, the vast majority of datasets showed no meaningful differences in predictive performance across the considered values of MAX\_DEPTH\_ROOT for any of the performance metrics. In a few datasets, however, a noticeable deterioration in performance was observed for larger MAX\_DEPTH\_ROOT values in terms of **Brier**. This deterioration increased steadily up to a depth of 5 and then appeared to plateau. The decline in performance for the default value of 3 compared with the best-performing value of 2 was small.

An informal analysis further indicated that datasets exhibiting such deterioration for larger depths tended to be small (results not shown). For AUC and ACC, only one dataset showed a clear

decline in performance with increasing depth. Overall, these findings suggest that the default value `MAX_DEPTH_ROOT = 3` is appropriate, as it provides predictive performance that is equal to or very close to the optimal value for most datasets.

For the proportion of covariates `PROP_VAR` sampled for each tree root, we used the default value  $\sqrt{p}/p$  for  $p \leq 100$ . Sampling only a subset of the covariates promotes diversity among the tree roots and prevents domination by a few covariates with strong marginal effects. To assess whether smaller or larger values yield better predictive performance, we examined the following grid for `PROP_VAR`:  $0.5\sqrt{p}/p$ ,  $\sqrt{p}/p$ ,  $2\sqrt{p}/p$ ,  $3\sqrt{p}/p$ ,  $4\sqrt{p}/p$ , and 1, where values exceeding 1 were set to 1.

The overall pattern closely mirrors that observed for `N_CAND_TREES` and `MAX_DEPTH_ROOT`: for the vast majority of datasets, predictive performance was virtually unchanged across the range of `PROP_VAR` values (Figure S1). In terms of **Brier**, for some datasets, a small deterioration was observed between  $0.5\sqrt{p}/p$  and  $\sqrt{p}/p$ , as well as between  $\sqrt{p}/p$  and  $2\sqrt{p}/p$ . However, these differences were similarly minor as those observed for `MAX_DEPTH_ROOT`. From  $2\sqrt{p}/p$  onward, no notable differences in **Brier** were found.

For **AUC** and **ACC**, the results showed no consistent trend. Although small fluctuations were visible for low `PROP_VAR` values, these were negligible in magnitude except for one dataset, and there was no general tendency toward either improved or degraded performance with increasing `PROP_VAR`.

### B.3 Comparison of Dataset-Specific Performance Measure Values of UFOs and Conventional RFs

Figure S2 displays the dataset-specific performance measures achieved by UFOs plotted against those achieved by RFs. Across the vast majority of datasets, the performance differences between the two methods were small, with somewhat larger deviations in a few cases.

Apparent deviations in the range of small **Brier** values result from the axis transformation, which expands the lower end of the scale and thus visually amplifies small absolute differences. For the datasets in this low-**Brier** range—where such apparent deviations occur—the corresponding AUC values exceed 0.99, confirming that these datasets contain very strong predictive signals in the covariates.

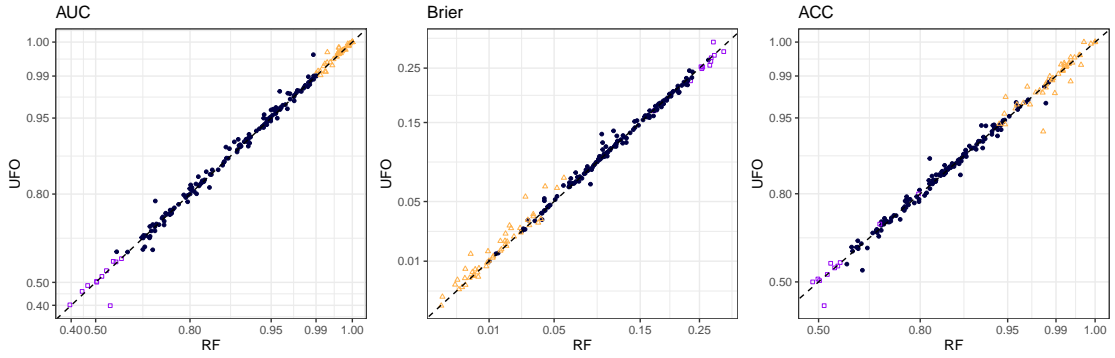

Fig. S2: Dataset-specific performance metric values: UFO versus conventional RF. Triangles represent datasets for which the AUC of both UFOs and conventional RFs was below 0.6, squares represent datasets with an AUC above 0.99 for both methods, and filled circles represent all remaining datasets. Axes were transformed for visual clarity: a square-root transformation was applied to Brier and a negative complementary square-root transformation was applied to AUC and ACC

## C Further Information on the Simulation Study

### C.1 Detailed Descriptions of the Covariate Effects Based on Simulated Datasets

This section provides detailed descriptions of Figures 1 and 2 from the main paper, which illustrate the empirical influences of the informative covariates in the two DGPs of the simulation study, based on exemplary simulated datasets.

#### C.1.1 DGP 1

Figure S3 (identical to Figure 1 in the main paper) shows the covariate values for all types of informative covariates in a dataset generated from DGP 1.

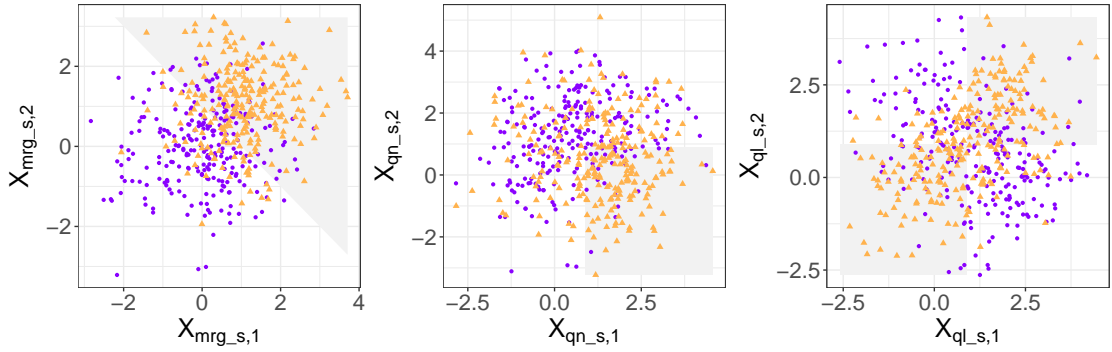

Fig. S3: Example pairs of variables with strong effects in a simulated dataset generated from DGP 1 ( $n = 500$ ). Circles and triangles represent observations from class 1 and 2, respectively. Shaded regions indicate areas of the covariate space with an above-average concentration of observations from class 2

The left panel displays a scatter plot of two covariates with purely marginal effects. These covariates, denoted  $X_{mrg\_s}$ , have strong marginal effects: as  $X_{mrg\_s}$  increases, the probability of belonging to class 2 increases correspondingly.

The middle panel in Figure S3 shows an interacting pair of covariates with marginal effects. For small values of  $X_{qn\_s,1}$ ,  $X_{qn\_s,2}$  has no effect—both classes are equally likely regardless of the value of  $X_{qn\_s,2}$ . In contrast, for large values of  $X_{qn\_s,1}$ , the probability of class 2 increases as  $X_{qn\_s,2}$  decreases. A similar pattern holds when interchanging the roles of  $X_{qn\_s,1}$  and  $X_{qn\_s,2}$ , confirming the presence of an interaction between these covariates. Their marginal effects are reflected in the fact that the expected probability for class 2 increases with larger values of either covariate. This pair, referred to as  $X_{qn\_s}$ , has a strong effect. The abbreviation “qn” stands for *quantitative*, as these covariates exhibit quantitative interaction effects—that is, interactions in which the strength, but not the direction, of one covariate’s effect depends on the value of the other.

The right panel of Figure S3 shows an interacting covariate pair without marginal effects. For small values of  $X_{ql\_s,1}$ , the probability for class 2 decreases as  $X_{ql\_s,2}$  increases, whereas for large values of  $X_{ql\_s,1}$ , the opposite holds: the probability for class 2 increases with larger  $X_{ql\_s,2}$  values.

Neither  $X_{ql,s,1}$  nor  $X_{ql,s,2}$  exhibit marginal effects, as the expected probability for class 2 does not change when the values of either variable are varied individually. This pair, denoted  $X_{ql,s}$ , has a strong effect. The abbreviation “ql” stands for *qualitative*, indicating qualitative interaction effects in which both the strength and the direction of one covariate’s effect depend on the value of the other.

### C.1.2 DGP 2

Figure S4 (identical to Figure 2 in the main paper) shows the empirical effects of the interacting covariates in a dataset generated from DGP 2.

The binary covariate  $X_{bne,ql}$  and the continuous covariate  $X_{ql,bne,s}$  exhibit an interaction effect in which neither covariate has a marginal effect. In the case of  $X_{bne,ql}$ , the class frequencies do not differ between its two categories. For  $X_{bne,ql} = 0$ ,  $X_{ql,bne,s}$  has a strongly positive effect on the probability of class 2, while for  $X_{bne,ql} = 1$ , it has a strongly negative effect—indicating a qualitative interaction.

The pair  $\{X_{be,ql}, X_{ql,be,s}\}$  exhibits an analogous interaction effect, except that  $X_{be,ql}$  has a moderate marginal effect: the probability for class 2 is higher for  $X_{be,ql} = 0$  than for  $X_{be,ql} = 1$ .

The interaction between the binary covariate  $X_{bne,qn}$  and the continuous covariate  $X_{qn,bne,s}$  is similar to that between  $X_{bne,ql}$  and  $X_{ql,bne,s}$ , but with a *quantitative* rather than a qualitative interaction. Moreover, unlike  $X_{ql,bne,s}$ ,  $X_{qn,bne,s}$  has a marginal effect. For  $X_{bne,qn} = 0$ ,  $X_{qn,bne,s}$  has no influence on class probabilities, whereas for  $X_{bne,qn} = 1$ , it has a strongly positive effect on the probability for class 2.

Finally, the categorical covariate  $X_{cne,ql}$  (with three categories) and the continuous covariate  $X_{ql,cne,s}$  show a qualitative interaction effect, again without marginal effects. For  $X_{cne,ql} = 1$ ,  $X_{ql,cne,s}$  strongly increases the probability for class 2; for  $X_{cne,ql} = 3$ , it strongly decreases it; and for  $X_{cne,ql} = 2$ , it has no influence.

## C.2 Formal Descriptions of the DGPs

In this section, we provide formal descriptions of the two DGPs used in the simulation study.

### C.2.1 DGP 1

The following detailed description follows Section E.2 of Supplementary Material 1 of Hornung and Boulesteix (2022) and is reproduced here almost verbatim for completeness.

For each simulated dataset the first  $n/2$  observations are from the first class and the second  $n/2$  observations are from the second class. The distributions from which the values of the informative covariates were drawn differ between the two classes.

The values of the 50 uninformative covariates were drawn from the standard normal distribution  $\mathcal{N}(0, 1)$ .

The values of the covariates  $X_{mrg,s}$ ,  $X_{mrg,m}$ , and  $X_{mrg,w}$  with only marginal effects, but no interaction effects were drawn from  $\mathcal{N}(0, 1)$  for observations from the first class and from  $\mathcal{N}(d, 1)$  for observations from the second class, where  $d = 1$  for covariates with strong effects,  $d = 0.75$  for covariates with moderate effects, and  $d = 0.5$  for covariates with weak effects (compare also Janitz et al. (2013)).

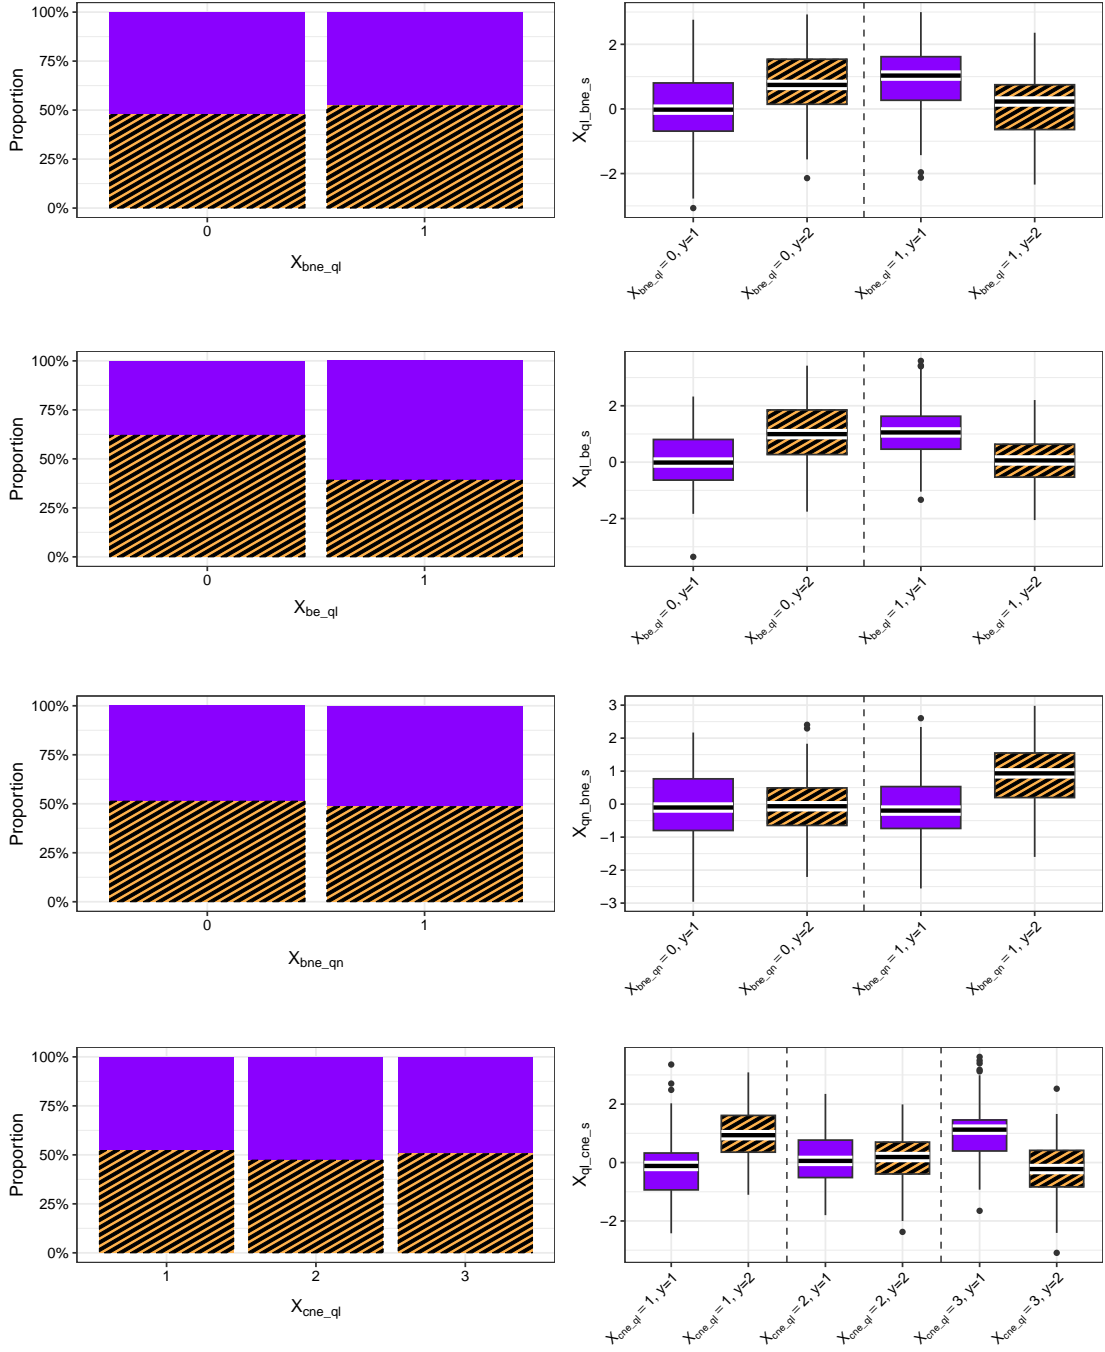

Fig. S4: Empirical effects of the interacting covariates in a simulated dataset generated from DGP 2 ( $n = 500$ ). In the bar plots, solid and hatched areas represent the proportions of classes 1 and 2, respectively. In the box plots, solid and hatched boxes correspond to the covariate values of classes 1 and 2, respectively

Be  $V$  the covariate space spanned by two continuous covariates  $X_1^*$  and  $X_2^*$ , where  $X_1^*$  is on the x-axis and  $X_2^*$  is on the y-axis. In the following, when referring to  $V$ , the covariate named first

corresponds to  $X_1^*$  and the covariate name second corresponds to  $X_2^*$ . The values of the covariate pairs with qualitative interactions  $\{X_{ql-s,1}, X_{ql-s,2}\}$ ,  $\{X_{ql-m,1}, X_{ql-m,2}\}$ , and  $\{X_{ql-w,1}, X_{ql-w,2}\}$  were drawn in such a way that the values from one class concentrate in the lower-left and upper-right corner of  $V$  and the values from the other class concentrate in the upper-left and lower-right corner of  $V$ . More precisely, the values of the covariate pairs were drawn from the following mixtures of multivariate normal distributions:

For  $\{X_{ql-m,1}, X_{ql-m,2}\}$  the values in the first class and for  $\{X_{ql-s,1}, X_{ql-s,2}\}$  and  $\{X_{ql-w,1}, X_{ql-w,2}\}$  the values in the second class were drawn from the following distribution:

$$\frac{1}{2} \cdot \mathcal{N} \left[ \begin{pmatrix} 0 \\ 0 \end{pmatrix}, \begin{pmatrix} 1 & 0 \\ 0 & 1 \end{pmatrix} \right] + \frac{1}{2} \cdot \mathcal{N} \left[ \begin{pmatrix} a \\ a \end{pmatrix}, \begin{pmatrix} 1 & 0 \\ 0 & 1 \end{pmatrix} \right] \quad (5)$$

For  $\{X_{ql-m,1}, X_{ql-m,2}\}$  the values in the second class and for  $\{X_{ql-s,1}, X_{ql-s,2}\}$  and  $\{X_{ql-w,1}, X_{ql-w,2}\}$  the values in the first class were drawn from the following distribution:

$$\frac{1}{2} \cdot \mathcal{N} \left[ \begin{pmatrix} a \\ 0 \end{pmatrix}, \begin{pmatrix} 1 & 0 \\ 0 & 1 \end{pmatrix} \right] + \frac{1}{2} \cdot \mathcal{N} \left[ \begin{pmatrix} 0 \\ a \end{pmatrix}, \begin{pmatrix} 1 & 0 \\ 0 & 1 \end{pmatrix} \right] \quad (6)$$

As will be described in the following, the values of the parameter  $a$  for strong, moderate, and weak qualitative interaction effects were specified in such a way that the resulting covariates featured a comparable predictive power as the covariates with only marginal effects of the same effect strength levels. In a general context, the predictive importance of a covariate is not only determined by how decisive the covariate is on its own, but also by how predictive the covariate is in conjunction with other covariates. For example, two predictive covariates, when considered together, may deliver a very accurate prediction rule, but when considered separately the two covariates may not be nearly as predictive. Thus, the predictive importance of one of these covariates depends on the presence of the other covariate. If we want to measure the predictive importance of a covariate, it is necessary to study how important this covariate is in conjunction with other covariates in the mean. The predictive importance of two covariates can be measured in terms of the similarity or dissimilarity of the joint distributions of these covariates in the two classes. The more similar these joint distributions are between the two classes, the less predictive power is featured in these covariates. The similarity between two probability density functions  $f_A(\mathbf{x})$  and  $f_B(\mathbf{x})$  can be measured using the overlapping index (Pastore and Calcagni, 2019):  $\int \min[f_A(\mathbf{x}), f_B(\mathbf{x})] d\mathbf{x} \in [0, 1]$ . We used this overlapping index for making the predictive powers of the covariates with qualitative interaction effects comparable to that of the covariates with only marginal effects of the same effect strength levels. This is realized by choosing values for parameter  $a$  that lead to degrees of overlap between the joint distributions of the interacting covariates in the two classes that are comparable to the corresponding overlaps for pairs of covariates for which one or both of them have a univariable effect. Denote  $\theta \in \{\text{strong}, \text{moderate}, \text{weak}\}$  the effect strength,  $\{X_{\theta,q,1}, X_{\theta,q,2}\}$  a covariate pair with qualitative interaction effect of strength  $\theta$ ,  $X_{\theta,u}$  a covariate with univariable effect of strength  $\theta$ ,  $X_{\theta,Un \setminus u,1}, \dots, X_{\theta,Un \setminus u,5}$  all covariates with univariable effect with the exception of  $X_{\theta,u}$ , and  $X_{\theta,No,1}, \dots, X_{\theta,No,50}$  all covariates without effect. Moreover, let  $O(X_{j_1}, X_{j_2})$  denote the overlapping index between the joint distributions of a covariate pair  $\{X_{j_1}, X_{j_2}\}$  in the two classes. Then for each effect strength

level  $\theta \in \{strong, moderate, weak\}$ , the parameter  $a$  in formulas (5) and (6) was fixed to the value for which the following equation holds:  $O(X_{\theta,q,1}, X_{\theta,q,2}) = \frac{1}{55} \sum_{X_j \in S_{\setminus u}} O(X_{\theta,u}, X_j)$ , where  $S_{\setminus u} = \{X_{\theta,Un \setminus u,1}, \dots, X_{\theta,Un \setminus u,5}, X_{\theta,No,1}, \dots, X_{\theta,No,50}\}$ . The reason why we did not include the covariates that feature interaction effects in these averages was simplicity: If we had included these covariates, the parameter controlling the overlapping index for pairs of covariates with quantitative interactions (see below) would have depended on the value of  $a$  and vice versa. This would have made it difficult to find the correct values of these parameters. We calculated each overlapping index value numerically with an exactness of three decimal places. The following  $a$  values resulted for strong, moderate, and weak effects: 1.772, 1.51, and 1.225.

The values of the covariate pairs with quantitative interactions  $\{X_{qn-s,1}, X_{qn-s,2}\}$ ,  $\{X_{qn-m,1}, X_{qn-m,2}\}$ , and  $\{X_{qn-w,1}, X_{qn-w,2}\}$  were drawn in such a way that the values from the second class concentrate in one corner of  $V$  and the values of the first class are distributed across the remaining three corners of  $V$ . For  $\{X_{qn-s,1}, X_{qn-s,2}\}$  the values of the second class concentrate in the lower-right corner, for  $\{X_{qn-m,1}, X_{qn-m,2}\}$  in the upper-right corner, and for  $\{X_{qn-w,1}, X_{qn-w,2}\}$  in the upper-left corner. Below we will demonstrate how the values of  $\{X_{qn-s,1}, X_{qn-s,2}\}$  were drawn. The values of  $\{X_{qn-m,1}, X_{qn-m,2}\}$  and  $\{X_{qn-w,1}, X_{qn-w,2}\}$  were drawn analogously with the difference that for these the values in the second class concentrate in a different corner of  $V$ . The values of  $\{X_{qn-s,1}, X_{qn-s,2}\}$  in the first class were drawn from the following distribution:

$$\frac{1}{3} \cdot \mathcal{N} \left[ \begin{pmatrix} 0 \\ a \end{pmatrix}, \begin{pmatrix} 1 & 0 \\ 0 & 1 \end{pmatrix} \right] + \frac{1}{3} \cdot \mathcal{N} \left[ \begin{pmatrix} a \\ a \end{pmatrix}, \begin{pmatrix} 1 & 0 \\ 0 & 1 \end{pmatrix} \right] + \frac{1}{3} \cdot \mathcal{N} \left[ \begin{pmatrix} 0 \\ 0 \end{pmatrix}, \begin{pmatrix} 1 & 0 \\ 0 & 1 \end{pmatrix} \right] \quad (7)$$

The values of  $\{X_{qn-s,1}, X_{qn-s,2}\}$  in the second class were drawn from the following distribution:

$$\begin{aligned} & \pi_a \cdot \mathcal{N} \left[ \begin{pmatrix} a \\ 0 \end{pmatrix}, \begin{pmatrix} 1 & 0 \\ 0 & 1 \end{pmatrix} \right] + \frac{1 - \pi_a}{3} \cdot \mathcal{N} \left[ \begin{pmatrix} 0 \\ a \end{pmatrix}, \begin{pmatrix} 1 & 0 \\ 0 & 1 \end{pmatrix} \right] + \\ & \frac{1 - \pi_a}{3} \cdot \mathcal{N} \left[ \begin{pmatrix} a \\ a \end{pmatrix}, \begin{pmatrix} 1 & 0 \\ 0 & 1 \end{pmatrix} \right] + \frac{1 - \pi_a}{3} \cdot \mathcal{N} \left[ \begin{pmatrix} 0 \\ 0 \end{pmatrix}, \begin{pmatrix} 1 & 0 \\ 0 & 1 \end{pmatrix} \right] \end{aligned} \quad (8)$$

Here,  $a$  is fixed to the same value 1.772 that was also used in the case of  $\{X_{ql-s,1}, X_{ql-s,2}\}$ , that is, the covariate pair with strong qualitative interaction effect. The larger the value of  $\pi_a$  is, the greater is the concentration of the second class in the lower-right corner. We fixed  $\pi_a$  to that value for which the overlapping index between the two class-specific joint distributions of  $\{X_{qn-s,1}, X_{qn-s,2}\}$  took the same value as that for  $\{X_{ql-s,1}, X_{ql-s,2}\}$ . An obvious alternative to this proceeding would have been to fix  $\pi_a$  to the value one and alter the value of  $a$  for achieving the desired overlapping index instead of diminishing the concentration of observations in the lower-right corner until the desired value of the overlapping index was achieved. However, this procedure would have led to a too small  $a$  value, because for quantitative interaction effects the covariate value pairs in the second class vary less than in the case of qualitative interaction effects. As a consequence, the means of the normal mixture components in equations (7) and (8) associated with the same overlapping index value as in the case of the strong qualitative interaction effect would have been close to each other. The following  $\pi_a$  values resulted for strong, moderate, and weak effects: 0.649, 0.574, and 0.485. The same  $a$  values (1.772, 1.51, and 1.225) as in the case of

the qualitative interaction effects were used for the three effect strength levels.

### C.2.2 DGP 2

As in DGP 1, the first  $n/2$  observations belong to class 1 and the remaining  $n/2$  to class 2. The non-informative covariates were generated analogously to those in DGP 1, drawn from the standard normal distribution  $\mathcal{N}(0, 1)$ .

In the following, let  $Y \in 1, 2$  denote the binary outcome. The informative covariates were simulated as follows:

1. Covariates  $X_{mrg\_s}$ ,  $X_{mrg\_m}$  and  $X_{mrg\_w}$ :

$$X_{mrg\_s} \mid Y = 1 \sim \mathcal{N}(0, 1), \quad X_{mrg\_s} \mid Y = 2 \sim \mathcal{N}(d = 1, 1).$$

$X_{mrg\_m}$  and  $X_{mrg\_w}$  were generated analogously, with  $d = 0.75$  and  $d = 0.5$ , respectively.

2. Covariates  $X_{bne\_ql}$ ,  $X_{ql\_bne\_s}$ ,  $X_{ql\_bne\_m}$  and  $X_{ql\_bne\_w}$ :

$$X_{bne\_ql} \sim \text{Bernoulli}(0.5).$$

If  $X_{bne\_ql} = 0$ :

$$X_{ql\_bne\_s} \mid Y = 1 \sim \mathcal{N}(0, 1), \quad X_{ql\_bne\_s} \mid Y = 2 \sim \mathcal{N}(d = 1, 1).$$

If  $X_{bne\_ql} = 1$ :

$$X_{ql\_bne\_s} \mid Y = 1 \sim \mathcal{N}(d = 1, 1), \quad X_{ql\_bne\_s} \mid Y = 2 \sim \mathcal{N}(0, 1).$$

$X_{ql\_bne\_m}$  and  $X_{ql\_bne\_w}$  were generated analogously to  $X_{ql\_bne\_s}$ , with  $d = 0.75$  and  $d = 0.5$ , respectively.

3. Covariates  $X_{be\_ql}$ ,  $X_{ql\_be\_s}$ ,  $X_{ql\_be\_m}$ , and  $X_{ql\_be\_w}$ :

$$X_{be\_ql} \mid Y = 1 \sim \text{Bernoulli}(0.6), \quad X_{be\_ql} \mid Y = 2 \sim \text{Bernoulli}(0.4).$$

$X_{ql\_be\_s}$ ,  $X_{ql\_be\_m}$  and  $X_{ql\_be\_w}$  were generated analogously to  $X_{ql\_bne\_s}$ ,  $X_{ql\_bne\_m}$  and  $X_{ql\_bne\_w}$ , whereby  $X_{be\_ql}$  was used instead of  $X_{bne\_ql}$ .

4. Covariates  $X_{bne\_qn}$ ,  $X_{qn\_bne\_s}$ ,  $X_{qn\_bne\_m}$ , and  $X_{qn\_bne\_w}$ :

$$X_{bne\_qn} \sim \text{Bernoulli}(0.5).$$

If  $X_{bne\_qn} = 0$ :

$$X_{qn\_bne\_s} \sim \mathcal{N}(0, 1).$$

If  $X_{bne\_qn} = 1$ :

$$X_{qn\_bne\_s} \mid Y = 1 \sim \mathcal{N}(0, 1), \quad X_{qn\_bne\_s} \mid Y = 2 \sim \mathcal{N}(d = 1, 1).$$

$X_{qn.bne.m}$  and  $X_{qn.bne.w}$  were generated analogously to  $X_{qn.bne.s}$ , where  $d = 0.75$  and  $d = 0.5$ , respectively.

5. Covariates  $X_{cne ql}$ ,  $X_{ql.cne.s}$ ,  $X_{ql.cne.m}$  and  $X_{ql.cne.w}$ :

$$P(X_{cne ql} = j) = \frac{1}{3}, \quad j = 1, 2, 3.$$

If  $X_{cne ql} = 1$ :

$$X_{ql.cne.s} \mid Y = 1 \sim \mathcal{N}(0, 1), \quad X_{ql.cne.s} \mid Y = 2 \sim \mathcal{N}(d = 1, 1).$$

If  $X_{cne ql} = 2$ :

$$X_{ql.cne.s} \sim \mathcal{N}(0, 1).$$

If  $X_{cne ql} = 3$ :

$$X_{ql.cne.s} \mid Y = 1 \sim \mathcal{N}(d = 1, 1), \quad X_{ql.cne.s} \mid Y = 2 \sim \mathcal{N}(0, 1).$$

$X_{ql.cne.m}$  and  $X_{ql.cne.w}$  were generated analogously to  $X_{ql.cne.s}$ , where  $d = 0.75$  and  $d = 0.5$ , respectively.

### C.3 Mean AUC Values With 95% Confidence Intervals and Median Ranks With 25% and 75% Quartiles

#### C.3.1 DGP 1

Table S6: Mean AUC values with 95% confidence intervals per considered sample size and method for DGP 1

| Covariate    | Method    | n = 100 |              | n = 300 |              | n = 500 |              | n = 1000 |              |
|--------------|-----------|---------|--------------|---------|--------------|---------|--------------|----------|--------------|
| $X_{mrg\_s}$ | Unity_vim | 0.46    | [0.45, 0.48] | 0.99    | [0.99, 1.00] | 1.00    | [1.00, 1.00] | 1.00     | [1.00, 1.00] |
|              | Perm      | 1.00    | [1.00, 1.00] | 1.00    | [1.00, 1.00] | 1.00    | [1.00, 1.00] | 1.00     | [1.00, 1.00] |
|              | Gini_corr | 1.00    | [0.99, 1.00] | 1.00    | [1.00, 1.00] | 1.00    | [1.00, 1.00] | 1.00     | [1.00, 1.00] |
| $X_{mrg\_m}$ | Unity_vim | 0.32    | [0.30, 0.33] | 0.84    | [0.83, 0.86] | 0.99    | [0.99, 1.00] | 1.00     | [1.00, 1.00] |
|              | Perm      | 0.98    | [0.97, 0.98] | 1.00    | [1.00, 1.00] | 1.00    | [1.00, 1.00] | 1.00     | [1.00, 1.00] |
|              | Gini_corr | 0.97    | [0.97, 0.98] | 1.00    | [1.00, 1.00] | 1.00    | [1.00, 1.00] | 1.00     | [1.00, 1.00] |
| $X_{mrg\_w}$ | Unity_vim | 0.36    | [0.34, 0.37] | 0.43    | [0.42, 0.45] | 0.69    | [0.67, 0.71] | 0.98     | [0.98, 0.99] |
|              | Perm      | 0.87    | [0.87, 0.88] | 0.99    | [0.99, 0.99] | 1.00    | [1.00, 1.00] | 1.00     | [1.00, 1.00] |
|              | Gini_corr | 0.87    | [0.85, 0.88] | 0.99    | [0.99, 0.99] | 1.00    | [1.00, 1.00] | 1.00     | [1.00, 1.00] |
| $X_{qn\_s}$  | Unity_vim | 0.34    | [0.32, 0.35] | 0.80    | [0.78, 0.81] | 0.98    | [0.98, 0.99] | 1.00     | [1.00, 1.00] |
|              | Perm      | 0.95    | [0.94, 0.95] | 1.00    | [1.00, 1.00] | 1.00    | [1.00, 1.00] | 1.00     | [1.00, 1.00] |
|              | Gini_corr | 0.93    | [0.93, 0.94] | 1.00    | [1.00, 1.00] | 1.00    | [1.00, 1.00] | 1.00     | [1.00, 1.00] |
| $X_{qn\_m}$  | Unity_vim | 0.35    | [0.34, 0.37] | 0.52    | [0.51, 0.54] | 0.83    | [0.81, 0.84] | 1.00     | [1.00, 1.00] |
|              | Perm      | 0.87    | [0.86, 0.88] | 0.99    | [0.99, 0.99] | 1.00    | [1.00, 1.00] | 1.00     | [1.00, 1.00] |
|              | Gini_corr | 0.86    | [0.85, 0.87] | 0.99    | [0.99, 0.99] | 1.00    | [1.00, 1.00] | 1.00     | [1.00, 1.00] |
| $X_{qn\_w}$  | Unity_vim | 0.41    | [0.39, 0.42] | 0.40    | [0.39, 0.42] | 0.50    | [0.48, 0.51] | 0.82     | [0.81, 0.83] |
|              | Perm      | 0.74    | [0.73, 0.75] | 0.93    | [0.92, 0.94] | 0.98    | [0.98, 0.99] | 1.00     | [1.00, 1.00] |
|              | Gini_corr | 0.74    | [0.73, 0.76] | 0.92    | [0.92, 0.93] | 0.98    | [0.97, 0.98] | 1.00     | [1.00, 1.00] |
| $X_{ql\_s}$  | Unity_vim | 0.67    | [0.65, 0.68] | 0.99    | [0.99, 1.00] | 1.00    | [1.00, 1.00] | 1.00     | [1.00, 1.00] |
|              | Perm      | 0.60    | [0.59, 0.62] | 0.76    | [0.75, 0.77] | 0.85    | [0.84, 0.85] | 0.96     | [0.96, 0.97] |
|              | Gini_corr | 0.52    | [0.50, 0.53] | 0.54    | [0.53, 0.56] | 0.56    | [0.54, 0.57] | 0.65     | [0.64, 0.66] |
| $X_{ql\_m}$  | Unity_vim | 0.54    | [0.52, 0.55] | 0.91    | [0.90, 0.92] | 0.99    | [0.99, 1.00] | 1.00     | [1.00, 1.00] |
|              | Perm      | 0.57    | [0.55, 0.58] | 0.67    | [0.66, 0.68] | 0.75    | [0.74, 0.76] | 0.88     | [0.87, 0.89] |
|              | Gini_corr | 0.51    | [0.50, 0.52] | 0.53    | [0.51, 0.54] | 0.56    | [0.54, 0.57] | 0.58     | [0.57, 0.60] |
| $X_{ql\_w}$  | Unity_vim | 0.49    | [0.48, 0.51] | 0.66    | [0.64, 0.67] | 0.85    | [0.84, 0.87] | 1.00     | [0.99, 1.00] |
|              | Perm      | 0.53    | [0.51, 0.54] | 0.59    | [0.57, 0.60] | 0.63    | [0.61, 0.64] | 0.72     | [0.71, 0.73] |
|              | Gini_corr | 0.50    | [0.49, 0.51] | 0.51    | [0.50, 0.52] | 0.52    | [0.51, 0.53] | 0.54     | [0.53, 0.56] |

Table S7: Median ranks with 25% and 75% quartiles per considered sample size and method for DGP 1

| Covariate    | Method    | n = 100     | n = 300     | n = 500     | n = 1000    |
|--------------|-----------|-------------|-------------|-------------|-------------|
| $X_{mrg\_s}$ | Unity_vim | 42 [5, 62]  | 2 [1, 3]    | 2 [1, 2]    | 2 [1, 2]    |
|              | Perm      | 2 [1, 3]    | 2 [1, 2]    | 2 [1, 2]    | 2 [1, 2]    |
|              | Gini_corr | 2 [1, 3]    | 2 [1, 2]    | 2 [1, 2]    | 2 [1, 2]    |
| $X_{mrg\_m}$ | Unity_vim | 53 [31, 65] | 7 [4, 16]   | 5 [3, 7]    | 4 [3, 5]    |
|              | Perm      | 5 [3, 8]    | 4 [3, 5]    | 4 [3, 5]    | 4 [3, 5]    |
|              | Gini_corr | 5 [3, 7]    | 4 [3, 5]    | 4 [3, 5]    | 4 [3, 5]    |
| $X_{mrg\_w}$ | Unity_vim | 48 [26, 61] | 47 [21, 63] | 19 [12, 49] | 13 [11, 15] |
|              | Perm      | 10 [6, 18]  | 9 [7, 10]   | 9 [7, 10]   | 9 [8, 10]   |
|              | Gini_corr | 9 [6, 18]   | 9 [7, 10]   | 9 [7, 10]   | 9 [7, 10]   |
| $X_{qn\_s}$  | Unity_vim | 50 [28, 63] | 9 [6, 26]   | 7 [4, 9]    | 5 [4, 7]    |
|              | Perm      | 6 [4, 10]   | 5 [4, 7]    | 5 [4, 6]    | 5 [4, 6]    |
|              | Gini_corr | 6 [4, 10]   | 6 [4, 7]    | 5 [4, 7]    | 5 [5, 6]    |
| $X_{qn\_m}$  | Unity_vim | 48 [27, 61] | 37 [13, 60] | 13 [10, 24] | 11 [9, 13]  |
|              | Perm      | 10 [6, 18]  | 8 [7, 10]   | 8 [7, 10]   | 8 [7, 9]    |
|              | Gini_corr | 9 [6, 18]   | 8 [7, 10]   | 8 [7, 10]   | 8 [7, 10]   |
| $X_{qn\_w}$  | Unity_vim | 42 [23, 57] | 48 [29, 61] | 43 [21, 61] | 18 [16, 30] |
|              | Perm      | 18 [10, 35] | 12 [10, 15] | 11 [10, 12] | 11 [11, 12] |
|              | Gini_corr | 17 [10, 35] | 11 [10, 14] | 11 [10, 12] | 11 [11, 12] |
| $X_{ql\_s}$  | Unity_vim | 17 [4, 39]  | 5 [3, 6]    | 6 [4, 7]    | 7 [6, 8]    |
|              | Perm      | 32 [21, 46] | 23 [17, 33] | 20 [15, 27] | 15 [14, 17] |
|              | Gini_corr | 38 [24, 53] | 37 [24, 52] | 36 [23, 51] | 28 [19, 44] |
| $X_{ql\_m}$  | Unity_vim | 30 [14, 49] | 8 [6, 12]   | 9 [8, 11]   | 11 [10, 12] |
|              | Perm      | 35 [21, 49] | 30 [20, 41] | 25 [18, 35] | 19 [16, 25] |
|              | Gini_corr | 39 [25, 53] | 38 [25, 53] | 36 [23, 51] | 34 [23, 49] |
| $X_{ql\_w}$  | Unity_vim | 34 [17, 49] | 24 [12, 45] | 14 [12, 24] | 15 [14, 16] |
|              | Perm      | 38 [25, 53] | 35 [24, 49] | 33 [22, 47] | 28 [20, 39] |
|              | Gini_corr | 40 [25, 54] | 40 [25, 54] | 39 [25, 53] | 37 [25, 53] |

### C.3.2 DGP 2

Table S8: Mean AUC values with 95% confidence intervals per considered sample size and method for DGP 2 (part 1)

| Covariate        | Method    | n = 100           | n = 300           | n = 500           | n = 1000          |
|------------------|-----------|-------------------|-------------------|-------------------|-------------------|
| $X_{mrg\_s}$     | Unity_vim | 0.45 [0.43, 0.48] | 0.99 [0.99, 1.00] | 1.00 [1.00, 1.00] | 1.00 [1.00, 1.00] |
|                  | Perm      | 1.00 [1.00, 1.00] | 1.00 [1.00, 1.00] | 1.00 [1.00, 1.00] | 1.00 [1.00, 1.00] |
|                  | Gini_corr | 1.00 [1.00, 1.00] | 1.00 [1.00, 1.00] | 1.00 [1.00, 1.00] | 1.00 [1.00, 1.00] |
| $X_{mrg\_m}$     | Unity_vim | 0.31 [0.29, 0.33] | 0.84 [0.82, 0.86] | 0.99 [0.99, 1.00] | 1.00 [1.00, 1.00] |
|                  | Perm      | 0.98 [0.97, 0.98] | 1.00 [1.00, 1.00] | 1.00 [1.00, 1.00] | 1.00 [1.00, 1.00] |
|                  | Gini_corr | 0.97 [0.97, 0.98] | 1.00 [1.00, 1.00] | 1.00 [1.00, 1.00] | 1.00 [1.00, 1.00] |
| $X_{mrg\_w}$     | Unity_vim | 0.36 [0.34, 0.38] | 0.43 [0.41, 0.46] | 0.68 [0.66, 0.71] | 0.98 [0.98, 0.99] |
|                  | Perm      | 0.87 [0.86, 0.88] | 0.99 [0.99, 0.99] | 1.00 [1.00, 1.00] | 1.00 [1.00, 1.00] |
|                  | Gini_corr | 0.86 [0.84, 0.87] | 0.99 [0.99, 1.00] | 1.00 [1.00, 1.00] | 1.00 [1.00, 1.00] |
| $X_{bne\_ql}$    | Unity_vim | 0.55 [0.53, 0.57] | 0.99 [0.98, 0.99] | 1.00 [1.00, 1.00] | 1.00 [1.00, 1.00] |
|                  | Perm      | 0.75 [0.75, 0.76] | 0.84 [0.84, 0.85] | 0.91 [0.90, 0.91] | 0.98 [0.98, 0.98] |
|                  | Gini_corr | 0.51 [0.50, 0.52] | 0.58 [0.57, 0.58] | 0.64 [0.63, 0.65] | 0.76 [0.75, 0.77] |
| $X_{ql\_bne\_s}$ | Unity_vim | 0.60 [0.58, 0.62] | 0.98 [0.97, 0.98] | 1.00 [1.00, 1.00] | 1.00 [1.00, 1.00] |
|                  | Perm      | 0.55 [0.53, 0.56] | 0.66 [0.65, 0.68] | 0.76 [0.75, 0.77] | 0.90 [0.89, 0.91] |
|                  | Gini_corr | 0.50 [0.49, 0.52] | 0.50 [0.49, 0.52] | 0.50 [0.48, 0.52] | 0.55 [0.53, 0.57] |
| $X_{ql\_bne\_m}$ | Unity_vim | 0.50 [0.48, 0.52] | 0.79 [0.77, 0.80] | 0.97 [0.96, 0.98] | 1.00 [1.00, 1.00] |
|                  | Perm      | 0.52 [0.50, 0.54] | 0.59 [0.57, 0.61] | 0.66 [0.65, 0.68] | 0.78 [0.77, 0.80] |
|                  | Gini_corr | 0.49 [0.48, 0.51] | 0.51 [0.50, 0.53] | 0.53 [0.51, 0.55] | 0.53 [0.51, 0.55] |
| $X_{ql\_bne\_w}$ | Unity_vim | 0.48 [0.46, 0.50] | 0.54 [0.52, 0.56] | 0.68 [0.66, 0.70] | 0.95 [0.94, 0.96] |
|                  | Perm      | 0.49 [0.48, 0.51] | 0.53 [0.52, 0.55] | 0.56 [0.54, 0.58] | 0.62 [0.60, 0.63] |
|                  | Gini_corr | 0.51 [0.49, 0.53] | 0.49 [0.47, 0.51] | 0.51 [0.49, 0.52] | 0.51 [0.49, 0.53] |
| $X_{be\_ql}$     | Unity_vim | 0.71 [0.68, 0.73] | 1.00 [1.00, 1.00] | 1.00 [1.00, 1.00] | 1.00 [1.00, 1.00] |
|                  | Perm      | 0.86 [0.86, 0.87] | 0.99 [0.98, 0.99] | 1.00 [1.00, 1.00] | 1.00 [1.00, 1.00] |
|                  | Gini_corr | 0.73 [0.72, 0.74] | 0.93 [0.92, 0.94] | 0.99 [0.98, 0.99] | 1.00 [1.00, 1.00] |
| $X_{ql\_be\_s}$  | Unity_vim | 0.58 [0.56, 0.60] | 0.97 [0.96, 0.98] | 1.00 [1.00, 1.00] | 1.00 [1.00, 1.00] |
|                  | Perm      | 0.67 [0.66, 0.69] | 0.94 [0.94, 0.95] | 1.00 [0.99, 1.00] | 1.00 [1.00, 1.00] |
|                  | Gini_corr | 0.52 [0.50, 0.54] | 0.77 [0.76, 0.79] | 0.94 [0.93, 0.95] | 1.00 [1.00, 1.00] |
| $X_{ql\_be\_m}$  | Unity_vim | 0.51 [0.49, 0.53] | 0.80 [0.78, 0.82] | 0.98 [0.97, 0.98] | 1.00 [1.00, 1.00] |
|                  | Perm      | 0.61 [0.60, 0.63] | 0.87 [0.86, 0.88] | 0.98 [0.98, 0.98] | 1.00 [1.00, 1.00] |
|                  | Gini_corr | 0.52 [0.50, 0.54] | 0.68 [0.67, 0.70] | 0.87 [0.86, 0.88] | 0.99 [0.99, 1.00] |
| $X_{ql\_be\_w}$  | Unity_vim | 0.49 [0.47, 0.51] | 0.54 [0.52, 0.56] | 0.69 [0.67, 0.71] | 0.95 [0.94, 0.96] |
|                  | Perm      | 0.55 [0.53, 0.56] | 0.74 [0.73, 0.76] | 0.89 [0.88, 0.90] | 0.99 [0.99, 0.99] |
|                  | Gini_corr | 0.51 [0.49, 0.53] | 0.58 [0.56, 0.60] | 0.73 [0.71, 0.75] | 0.94 [0.93, 0.94] |

Table S9: Mean AUC values with 95% confidence intervals per considered sample size and method for DGP 2 (part 2)

| Covariate        | Method    | n = 100 |              | n = 300 |              | n = 500 |              | n = 1000 |              |
|------------------|-----------|---------|--------------|---------|--------------|---------|--------------|----------|--------------|
| $X_{bne\_qn}$    | Unity_vim | 0.47    | [0.45, 0.49] | 0.54    | [0.52, 0.56] | 0.73    | [0.71, 0.75] | 0.97     | [0.96, 0.98] |
|                  | Perm      | 0.73    | [0.73, 0.74] | 0.79    | [0.78, 0.79] | 0.89    | [0.88, 0.89] | 0.99     | [0.99, 0.99] |
|                  | Gini_corr | 0.51    | [0.50, 0.52] | 0.59    | [0.58, 0.60] | 0.70    | [0.69, 0.70] | 0.89     | [0.89, 0.90] |
| $X_{qn\_bne\_s}$ | Unity_vim | 0.37    | [0.35, 0.39] | 0.80    | [0.78, 0.82] | 0.98    | [0.97, 0.98] | 1.00     | [1.00, 1.00] |
|                  | Perm      | 0.87    | [0.86, 0.88] | 0.99    | [0.99, 1.00] | 1.00    | [1.00, 1.00] | 1.00     | [1.00, 1.00] |
|                  | Gini_corr | 0.85    | [0.83, 0.86] | 0.99    | [0.98, 0.99] | 1.00    | [1.00, 1.00] | 1.00     | [1.00, 1.00] |
| $X_{qn\_bne\_m}$ | Unity_vim | 0.40    | [0.39, 0.42] | 0.53    | [0.51, 0.55] | 0.75    | [0.72, 0.77] | 0.99     | [0.99, 1.00] |
|                  | Perm      | 0.75    | [0.73, 0.77] | 0.94    | [0.93, 0.95] | 0.99    | [0.98, 0.99] | 1.00     | [1.00, 1.00] |
|                  | Gini_corr | 0.74    | [0.72, 0.76] | 0.93    | [0.92, 0.94] | 0.99    | [0.98, 0.99] | 1.00     | [1.00, 1.00] |
| $X_{qn\_bne\_w}$ | Unity_vim | 0.43    | [0.42, 0.45] | 0.43    | [0.41, 0.45] | 0.48    | [0.46, 0.51] | 0.75     | [0.73, 0.77] |
|                  | Perm      | 0.65    | [0.63, 0.67] | 0.82    | [0.80, 0.83] | 0.89    | [0.88, 0.90] | 0.98     | [0.98, 0.99] |
|                  | Gini_corr | 0.65    | [0.63, 0.67] | 0.81    | [0.79, 0.83] | 0.89    | [0.87, 0.90] | 0.98     | [0.98, 0.99] |
| $X_{cne\_ql}$    | Unity_vim | 0.48    | [0.46, 0.50] | 0.85    | [0.84, 0.87] | 0.99    | [0.98, 0.99] | 1.00     | [1.00, 1.00] |
|                  | Perm      | 0.73    | [0.72, 0.73] | 0.78    | [0.77, 0.79] | 0.85    | [0.84, 0.85] | 0.94     | [0.93, 0.94] |
|                  | Gini_corr | 0.51    | [0.49, 0.52] | 0.55    | [0.54, 0.56] | 0.60    | [0.59, 0.61] | 0.67     | [0.66, 0.68] |
| $X_{ql\_cne\_s}$ | Unity_vim | 0.50    | [0.49, 0.52] | 0.86    | [0.85, 0.88] | 0.98    | [0.98, 0.99] | 1.00     | [1.00, 1.00] |
|                  | Perm      | 0.54    | [0.52, 0.56] | 0.61    | [0.59, 0.63] | 0.68    | [0.67, 0.70] | 0.80     | [0.79, 0.81] |
|                  | Gini_corr | 0.52    | [0.50, 0.53] | 0.51    | [0.49, 0.52] | 0.52    | [0.50, 0.54] | 0.52     | [0.50, 0.54] |
| $X_{ql\_cne\_m}$ | Unity_vim | 0.49    | [0.47, 0.51] | 0.65    | [0.63, 0.67] | 0.85    | [0.83, 0.86] | 0.99     | [0.99, 1.00] |
|                  | Perm      | 0.52    | [0.51, 0.54] | 0.54    | [0.53, 0.56] | 0.60    | [0.58, 0.62] | 0.69     | [0.67, 0.70] |
|                  | Gini_corr | 0.49    | [0.47, 0.51] | 0.49    | [0.48, 0.51] | 0.52    | [0.50, 0.53] | 0.52     | [0.51, 0.54] |
| $X_{ql\_cne\_w}$ | Unity_vim | 0.48    | [0.46, 0.50] | 0.49    | [0.47, 0.51] | 0.56    | [0.54, 0.58] | 0.80     | [0.78, 0.82] |
|                  | Perm      | 0.50    | [0.48, 0.52] | 0.52    | [0.50, 0.54] | 0.55    | [0.53, 0.57] | 0.58     | [0.56, 0.59] |
|                  | Gini_corr | 0.50    | [0.49, 0.52] | 0.50    | [0.48, 0.52] | 0.51    | [0.49, 0.52] | 0.51     | [0.49, 0.53] |

Table S10: Median ranks with 25% and 75% quartiles per considered sample size and method for DGP 2 (part 1)

| Covariate        | Method    | n = 100     | n = 300     | n = 500     | n = 1000    |
|------------------|-----------|-------------|-------------|-------------|-------------|
| $X_{mrg\_s}$     | Unity_vim | 45 [8, 65]  | 2 [1, 3]    | 1 [1, 2]    | 1 [1, 1]    |
|                  | Perm      | 1 [1, 2]    | 1 [1, 1]    | 1 [1, 1]    | 1 [1, 1]    |
|                  | Gini_corr | 1 [1, 2]    | 1 [1, 1]    | 1 [1, 1]    | 1 [1, 1]    |
| $X_{mrg\_m}$     | Unity_vim | 57 [32, 66] | 7 [4, 17]   | 4 [3, 7]    | 3 [3, 4]    |
|                  | Perm      | 2 [2, 4]    | 2 [2, 2]    | 2 [2, 2]    | 2 [2, 2]    |
|                  | Gini_corr | 2 [2, 3]    | 2 [2, 2]    | 2 [2, 2]    | 2 [2, 2]    |
| $X_{mrg\_w}$     | Unity_vim | 49 [28, 63] | 49 [21, 64] | 18 [12, 52] | 12 [10, 14] |
|                  | Perm      | 6 [3, 14]   | 4 [3, 5]    | 4 [4, 5]    | 5 [4, 6]    |
|                  | Gini_corr | 6 [3, 14]   | 4 [3, 5]    | 4 [3, 4]    | 3 [3, 4]    |
| $X_{bne\_ql}$    | Unity_vim | 31 [11, 52] | 5 [4, 7]    | 5 [4, 6]    | 5 [5, 6]    |
|                  | Perm      | 23 [19, 26] | 19 [15, 23] | 16 [12, 19] | 12 [11, 14] |
|                  | Gini_corr | 37 [33, 41] | 34 [30, 39] | 32 [27, 36] | 25 [21, 30] |
| $X_{ql\_bne\_s}$ | Unity_vim | 25 [5, 49]  | 5 [4, 7]    | 6 [5, 8]    | 7 [6, 8]    |
|                  | Perm      | 37 [20, 50] | 29 [17, 42] | 24 [16, 34] | 17 [14, 22] |
|                  | Gini_corr | 38 [21, 53] | 38 [23, 55] | 41 [24, 56] | 38 [24, 51] |
| $X_{ql\_bne\_m}$ | Unity_vim | 35 [18, 53] | 12 [7, 31]  | 10 [8, 13]  | 11 [10, 13] |
|                  | Perm      | 38 [21, 53] | 34 [21, 49] | 30 [20, 43] | 24 [17, 34] |
|                  | Gini_corr | 38 [22, 55] | 39 [22, 53] | 39 [22, 53] | 39 [24, 55] |
| $X_{ql\_bne\_w}$ | Unity_vim | 36 [20, 52] | 37 [19, 54] | 25 [14, 46] | 16 [15, 18] |
|                  | Perm      | 41 [23, 55] | 40 [24, 52] | 38 [25, 52] | 35 [24, 47] |
|                  | Gini_corr | 36 [20, 53] | 41 [23, 55] | 40 [25, 55] | 41 [26, 55] |
| $X_{be\_ql}$     | Unity_vim | 10 [2, 40]  | 2 [1, 2]    | 2 [1, 2]    | 2 [2, 2]    |
|                  | Perm      | 13 [6, 20]  | 5 [3, 6]    | 3 [3, 5]    | 3 [3, 3]    |
|                  | Gini_corr | 22 [10, 32] | 7 [5, 12]   | 6 [5, 7]    | 6 [5, 6]    |
| $X_{ql\_be\_s}$  | Unity_vim | 28 [7, 48]  | 5 [4, 7]    | 6 [5, 8]    | 7 [6, 8]    |
|                  | Perm      | 24 [13, 39] | 8 [6, 11]   | 6 [6, 7]    | 6 [5, 6]    |
|                  | Gini_corr | 34 [19, 54] | 13 [9, 27]  | 8 [7, 10]   | 7 [6, 7]    |
| $X_{ql\_be\_m}$  | Unity_vim | 34 [16, 52] | 12 [8, 29]  | 10 [8, 12]  | 11 [10, 13] |
|                  | Perm      | 30 [16, 44] | 12 [9, 19]  | 8 [8, 10]   | 8 [7, 8]    |
|                  | Gini_corr | 34 [18, 54] | 21 [12, 39] | 11 [9, 17]  | 9 [8, 9]    |
| $X_{ql\_be\_w}$  | Unity_vim | 36 [20, 51] | 37 [20, 54] | 24 [14, 46] | 16 [14, 18] |
|                  | Perm      | 36 [19, 52] | 21 [13, 35] | 14 [10, 20] | 10 [9, 11]  |
|                  | Gini_corr | 36 [20, 54] | 31 [18, 50] | 19 [13, 33] | 11 [10, 13] |

Table S11: Median ranks with 25% and 75% quartiles per considered sample size and method for DGP 2 (part 2)

| Covariate        | Method    | n = 100     | n = 300     | n = 500     | n = 1000    |
|------------------|-----------|-------------|-------------|-------------|-------------|
| $X_{bne\_qn}$    | Unity_vim | 37 [22, 51] | 37 [21, 52] | 21 [13, 41] | 16 [14, 17] |
|                  | Perm      | 25 [21, 28] | 23 [18, 28] | 17 [13, 22] | 11 [10, 13] |
|                  | Gini_corr | 37 [32, 42] | 34 [29, 38] | 28 [22, 32] | 16 [13, 19] |
| $X_{qn\_bne\_s}$ | Unity_vim | 50 [25, 62] | 8 [4, 28]   | 5 [3, 8]    | 4 [3, 4]    |
|                  | Perm      | 6 [3, 15]   | 4 [3, 5]    | 4 [4, 5]    | 5 [4, 5]    |
|                  | Gini_corr | 6 [3, 15]   | 4 [3, 5]    | 4 [3, 4]    | 4 [3, 4]    |
| $X_{qn\_bne\_m}$ | Unity_vim | 43 [25, 60] | 37 [14, 59] | 14 [10, 42] | 9 [7, 13]   |
|                  | Perm      | 13 [5, 33]  | 6 [5, 10]   | 7 [5, 8]    | 7 [6, 8]    |
|                  | Gini_corr | 13 [5, 31]  | 5 [4, 8]    | 5 [5, 6]    | 5 [5, 7]    |
| $X_{qn\_bne\_w}$ | Unity_vim | 41 [22, 57] | 46 [28, 61] | 45 [25, 60] | 20 [16, 44] |
|                  | Perm      | 25 [9, 45]  | 12 [8, 27]  | 11 [8, 18]  | 9 [9, 11]   |
|                  | Gini_corr | 21 [9, 45]  | 10 [6, 24]  | 8 [7, 14]   | 8 [8, 9]    |
| $X_{cne\_ql}$    | Unity_vim | 37 [19, 54] | 10 [6, 20]  | 9 [7, 11]   | 9 [8, 11]   |
|                  | Perm      | 25 [21, 28] | 24 [19, 28] | 21 [16, 25] | 17 [14, 19] |
|                  | Gini_corr | 37 [31, 43] | 36 [31, 42] | 35 [29, 40] | 31 [26, 36] |
| $X_{ql\_cne\_s}$ | Unity_vim | 34 [17, 51] | 9 [6, 19]   | 9 [8, 11]   | 10 [9, 12]  |
|                  | Perm      | 37 [20, 51] | 34 [21, 47] | 29 [19, 42] | 22 [17, 32] |
|                  | Gini_corr | 36 [20, 52] | 39 [23, 55] | 39 [22, 54] | 40 [25, 54] |
| $X_{ql\_cne\_m}$ | Unity_vim | 36 [19, 53] | 27 [12, 47] | 14 [11, 27] | 14 [13, 16] |
|                  | Perm      | 38 [21, 53] | 38 [24, 52] | 35 [22, 48] | 30 [21, 42] |
|                  | Gini_corr | 38 [22, 55] | 41 [23, 55] | 40 [24, 53] | 40 [25, 53] |
| $X_{ql\_cne\_w}$ | Unity_vim | 36 [19, 52] | 40 [26, 55] | 38 [22, 54] | 20 [17, 36] |
|                  | Perm      | 39 [22, 56] | 41 [25, 54] | 39 [25, 53] | 37 [27, 52] |
|                  | Gini_corr | 37 [20, 55] | 39 [22, 56] | 40 [24, 55] | 41 [26, 55] |

## D Additional Results from the Empirical Evaluation of the CRTR Algorithm

### D.1 Simulated Data: Unity VIM and Permutation VIM Values

Figure S5 displays the 20 highest unity VIM and permutation VIM values for the two simulated datasets. In line with the results of the simulation study in Section 5 of the main paper, the unity VIM assigned considerably higher ranks to covariates involved in interaction effects without marginal effects, whereas the permutation VIM tended to rank covariates with weak marginal effects higher.

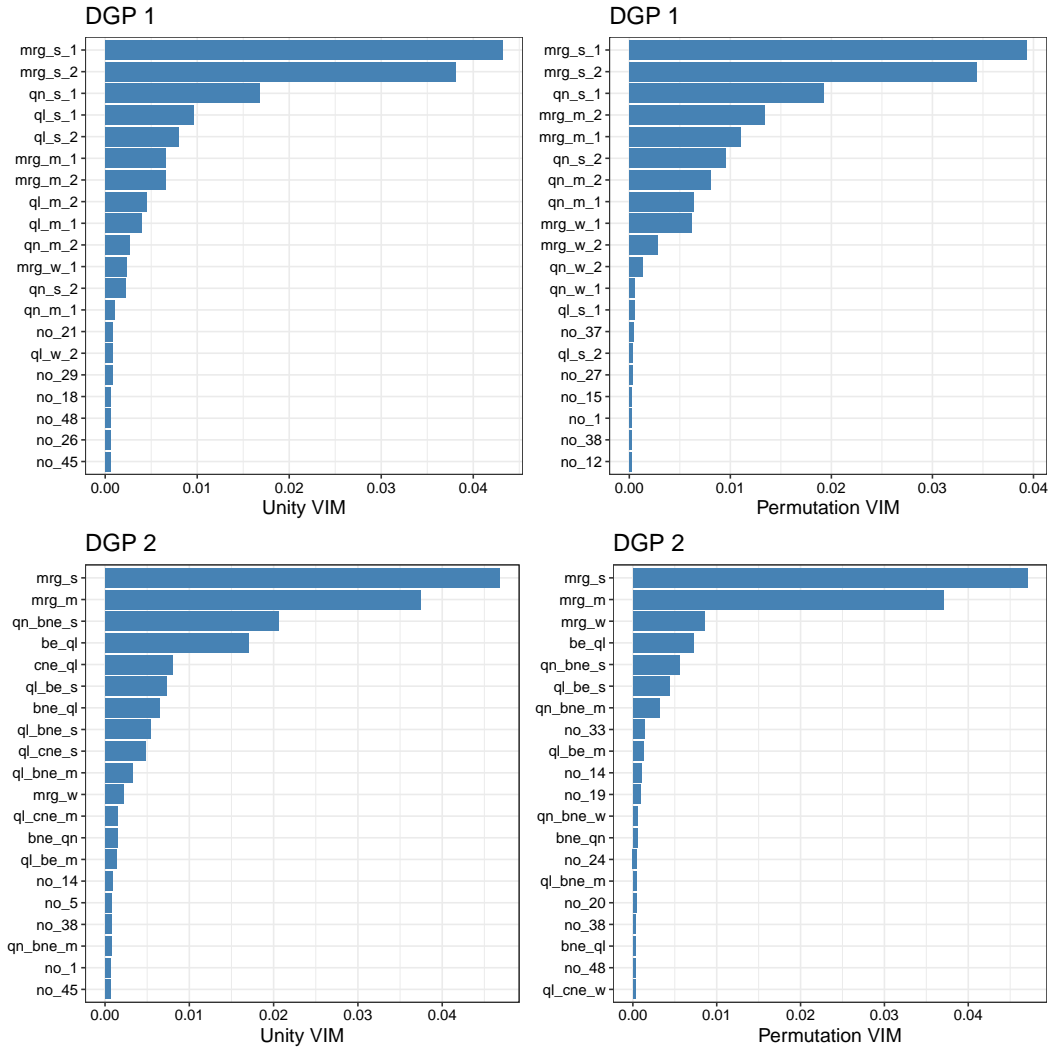

Fig. S5: Top 20 unity and permutation VIM values for one dataset each generated from DGP 1 and DGP 2 ( $n = 500$ )

## D.2 Simulated Data: CRTRs for all Informative Covariates

### D.2.1 DGP 1

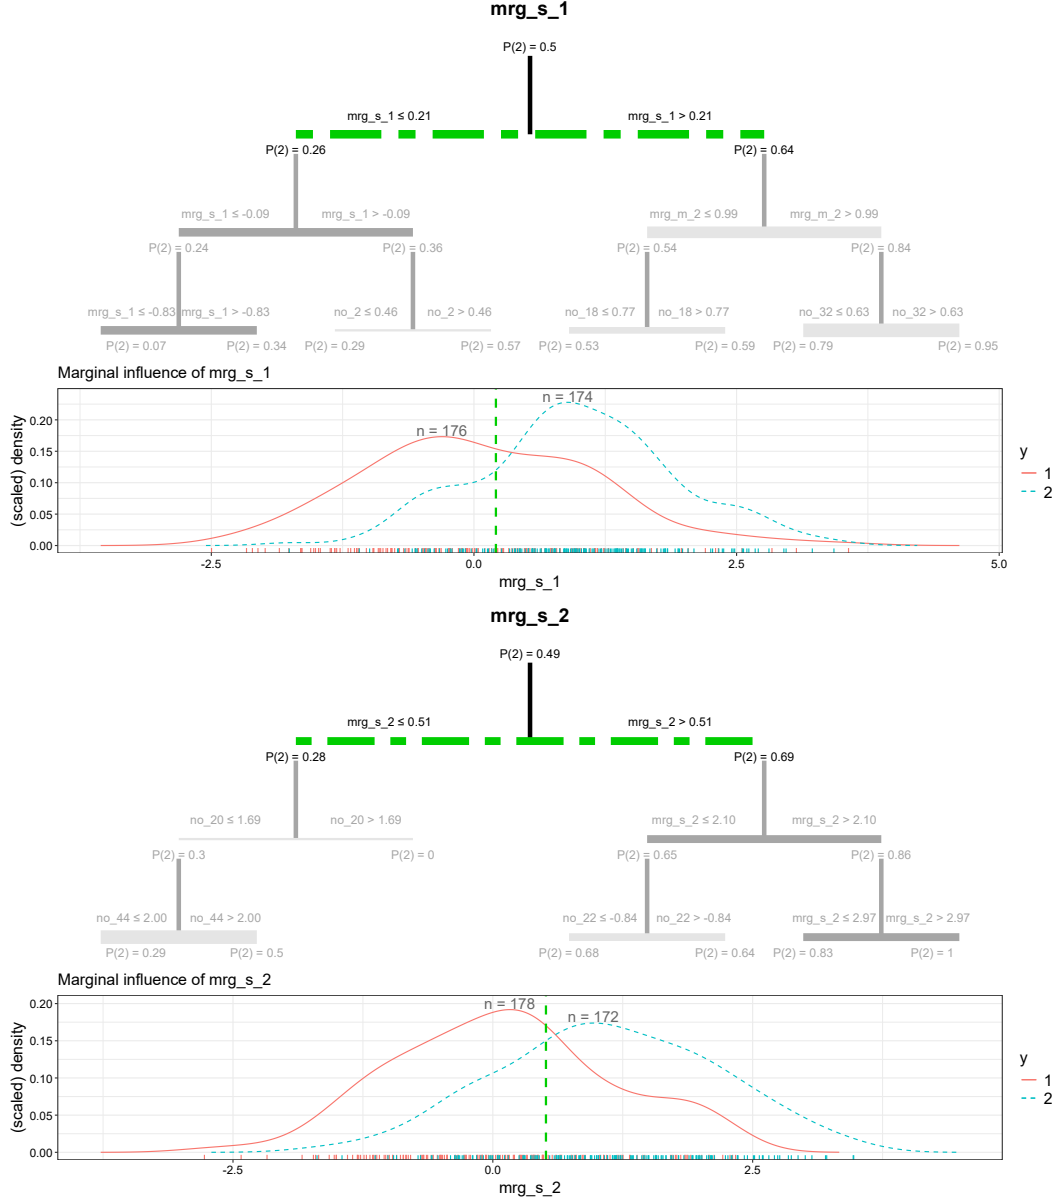

Fig. S6: Visualization of the CRTRs for the covariates  $X_{mrg\_s\_1}$  and  $X_{mrg\_s\_2}$  in a dataset generated from DGP 1 ( $n = 500$ ). The thickness of the horizontal lines reflects the covariate scores, dashed lines indicate top-scoring splits, and gray-shaded areas mark tree regions outside these splits and their ancestors. The class frequency distributions at the nodes and the weighted kernel density estimates of the class-specific covariate distributions were computed using the in-bag data.  $P(2)$  denotes the in-bag proportion of observations belonging to class 2 at the respective node. Covariate labels are abbreviated (e.g., **mrg\_m\_1** denotes  $X_{mrg\_m\_1}$  and **no\_\*** denotes non-informative covariates)

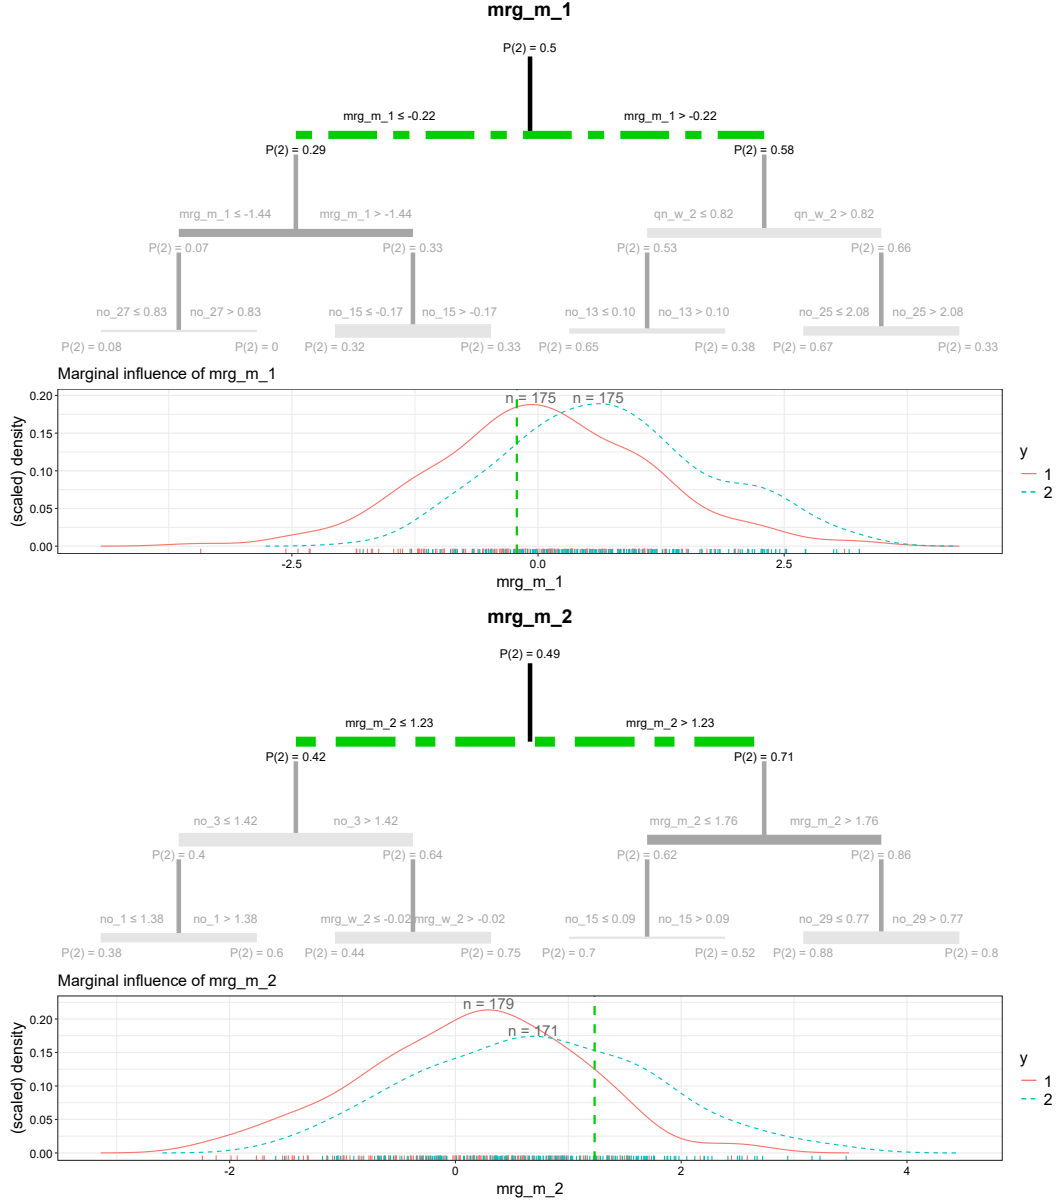

Fig. S7: Visualization of the CRTRs for the covariates  $X_{mrg-m.1}$  and  $X_{mrg-m.2}$  in a dataset generated from DGP 1 ( $n = 500$ ). The thickness of the horizontal lines reflects the covariate scores, dashed lines indicate top-scoring splits, and gray-shaded areas mark tree regions outside these splits and their ancestors. The class frequency distributions at the nodes and the weighted kernel density estimates of the class-specific covariate distributions were computed using the in-bag data.  $P(2)$  denotes the in-bag proportion of observations belonging to class 2 at the respective node. Covariate labels are abbreviated (e.g.,  $mrg\_m\_1$  denotes  $X_{mrg-m.1}$  and  $no\_*$  denotes non-informative covariates)

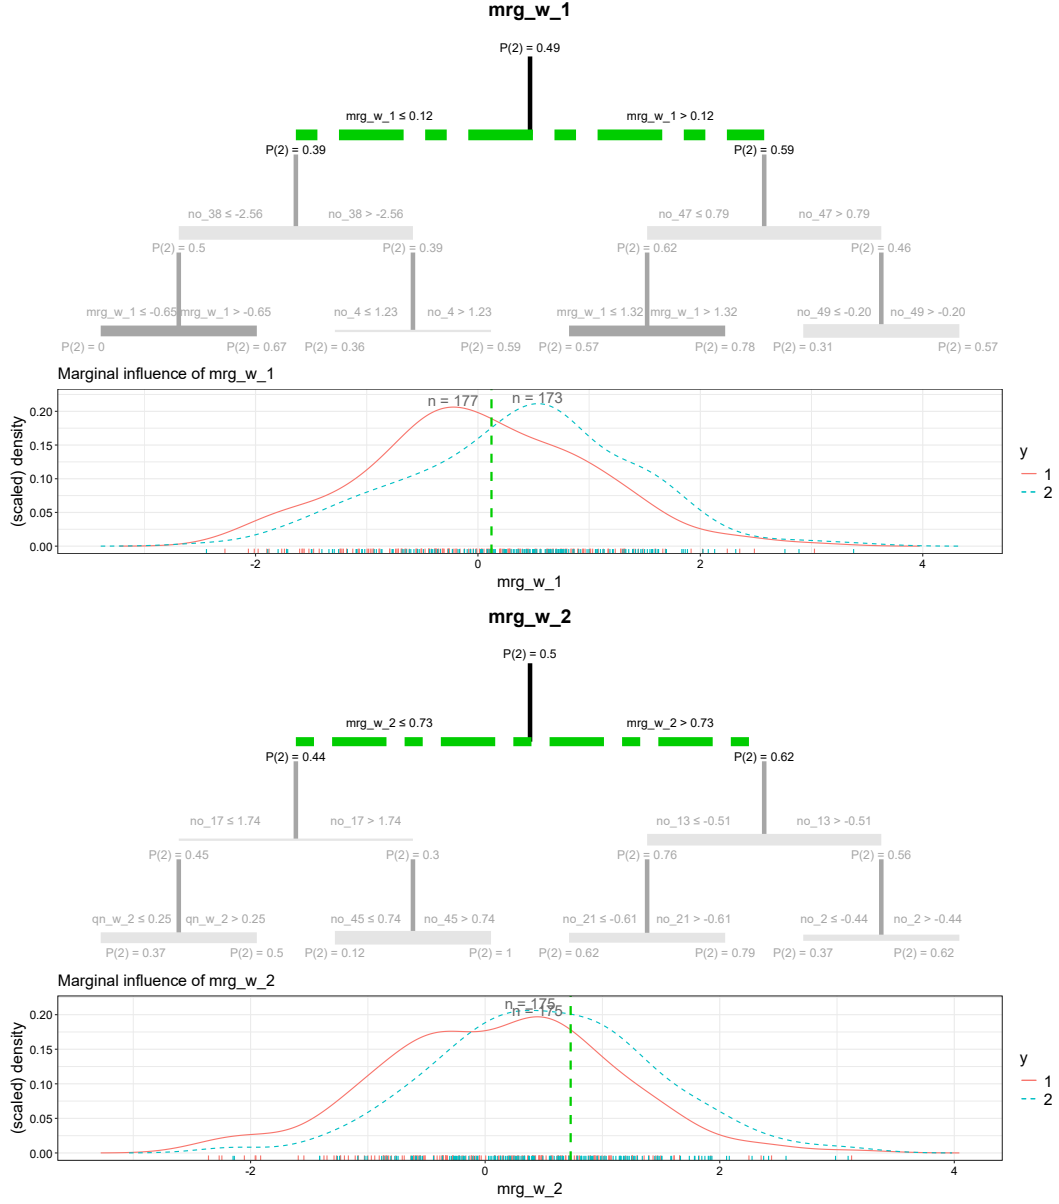

Fig. S8: Visualization of the CRTRs for the covariates  $X_{mrg-w-1}$  and  $X_{mrg-w-2}$  in a dataset generated from DGP 1 ( $n = 500$ ). The thickness of the horizontal lines reflects the covariate scores, dashed lines indicate top-scoring splits, and gray-shaded areas mark tree regions outside these splits and their ancestors. The class frequency distributions at the nodes and the weighted kernel density estimates of the class-specific covariate distributions were computed using the in-bag data.  $P(2)$  denotes the in-bag proportion of observations belonging to class 2 at the respective node. Covariate labels are abbreviated (e.g., **mrg\_w\_1** denotes  $X_{mrg-w-1}$  and **no.\*** denotes non-informative covariates)

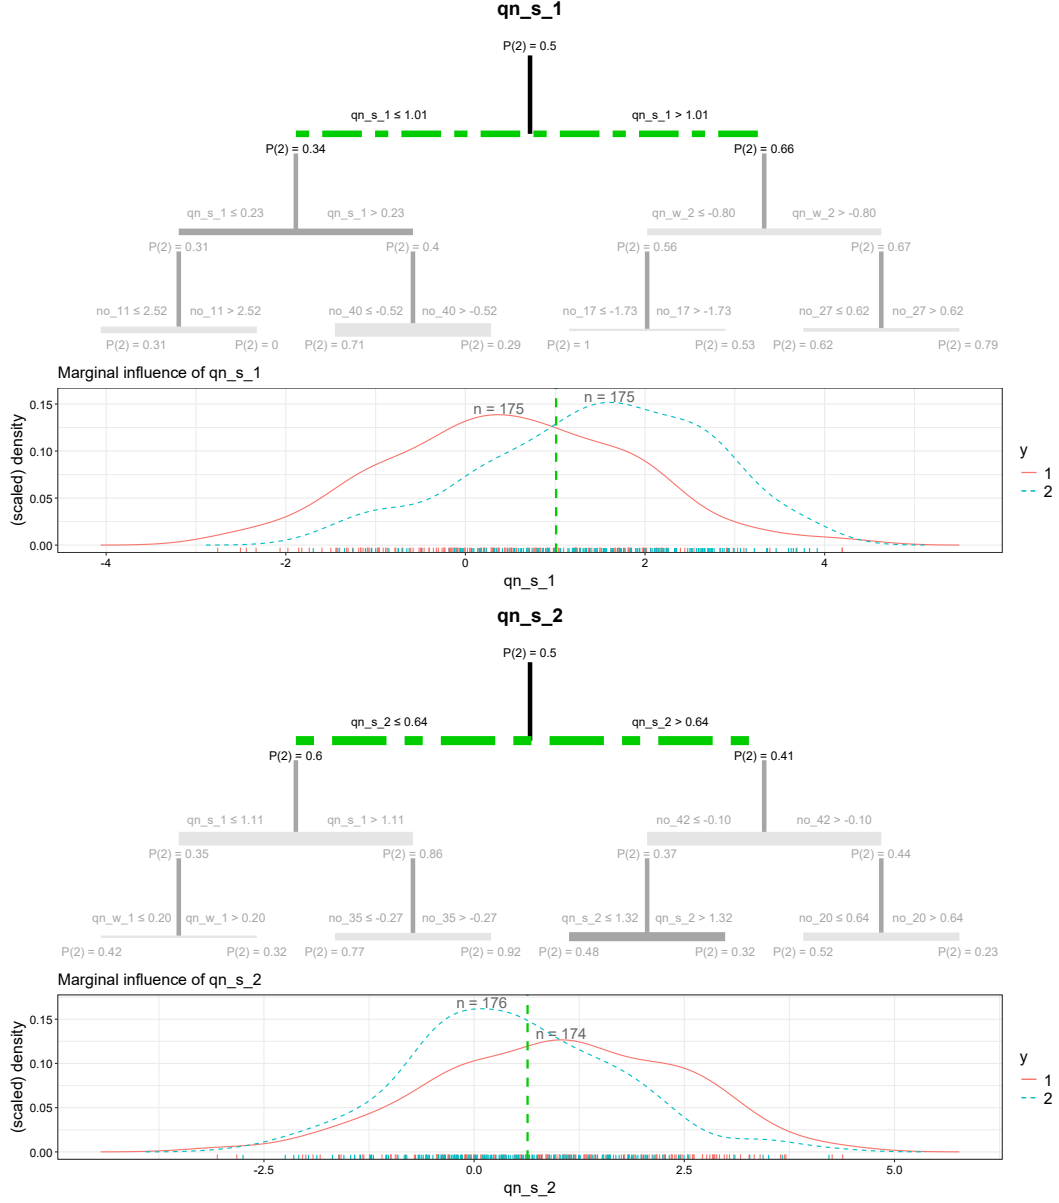

Fig. S9: Visualization of the CRTRs for the covariates  $X_{qn-s-1}$  and  $X_{qn-s-2}$  in a dataset generated from DGP 1 ( $n = 500$ ). The thickness of the horizontal lines reflects the covariate scores, dashed lines indicate top-scoring splits, and gray-shaded areas mark tree regions outside these splits and their ancestors. The class frequency distributions at the nodes and the weighted kernel density estimates of the class-specific covariate distributions were computed using the in-bag data.  $P(2)$  denotes the in-bag proportion of observations belonging to class 2 at the respective node. Covariate labels are abbreviated (e.g.,  $qn\_s\_1$  denotes  $X_{qn-s-1}$  and  $no\_*$  denotes non-informative covariates)

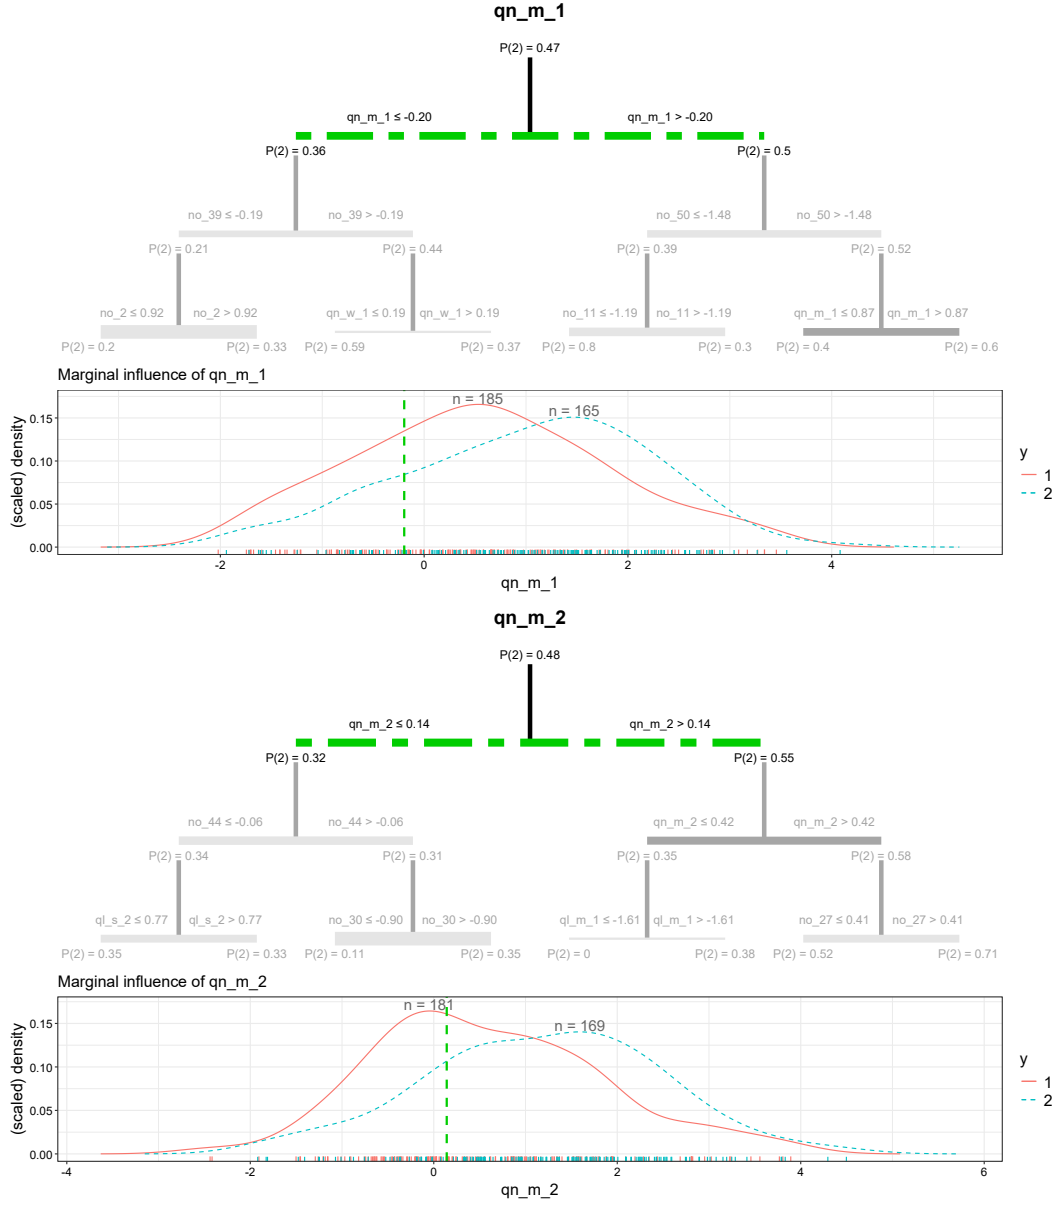

Fig. S10: Visualization of the CRTRs for the covariates  $X_{qn.m.1}$  and  $X_{qn.m.2}$  in a dataset generated from DGP 1 ( $n = 500$ ). The thickness of the horizontal lines reflects the covariate scores, dashed lines indicate top-scoring splits, and gray-shaded areas mark tree regions outside these splits and their ancestors. The class frequency distributions at the nodes and the weighted kernel density estimates of the class-specific covariate distributions were computed using the in-bag data.  $P(2)$  denotes the in-bag proportion of observations belonging to class 2 at the respective node. Covariate labels are abbreviated (e.g.,  $qn.m.1$  denotes  $X_{qn.m.1}$  and  $no.*$  denotes non-informative covariates)

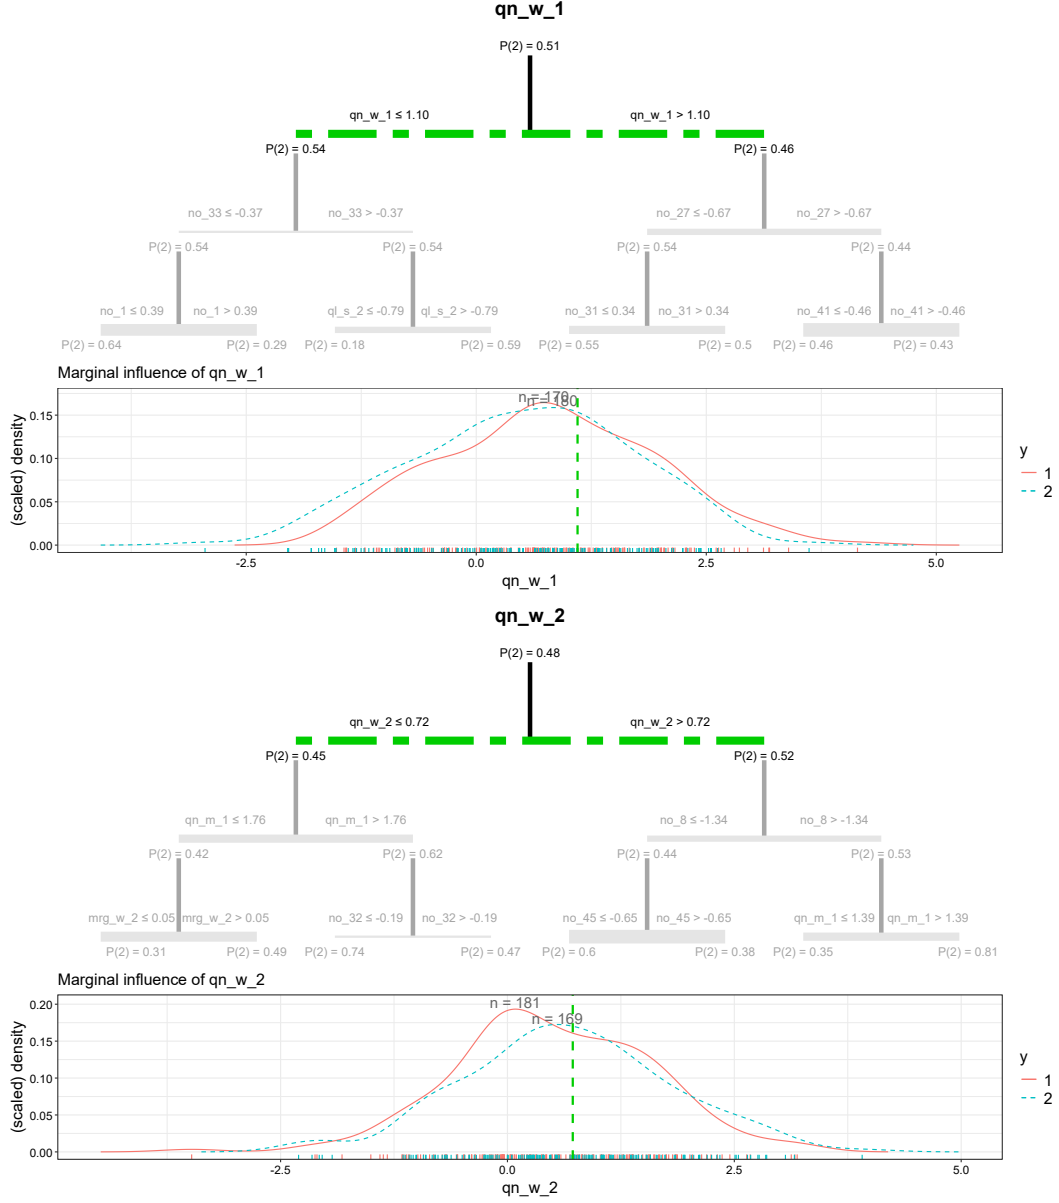

Fig. S11: Visualization of the CRTRs for the covariates  $X_{qn\_w\_1}$  and  $X_{qn\_w\_2}$  in a dataset generated from DGP 1 ( $n = 500$ ). The thickness of the horizontal lines reflects the covariate scores, dashed lines indicate top-scoring splits, and gray-shaded areas mark tree regions outside these splits and their ancestors. The class frequency distributions at the nodes and the weighted kernel density estimates of the class-specific covariate distributions were computed using the in-bag data.  $P(2)$  denotes the in-bag proportion of observations belonging to class 2 at the respective node. Covariate labels are abbreviated (e.g.,  $qn\_w\_1$  denotes  $X_{qn\_w\_1}$  and  $no\_*$  denotes non-informative covariates)

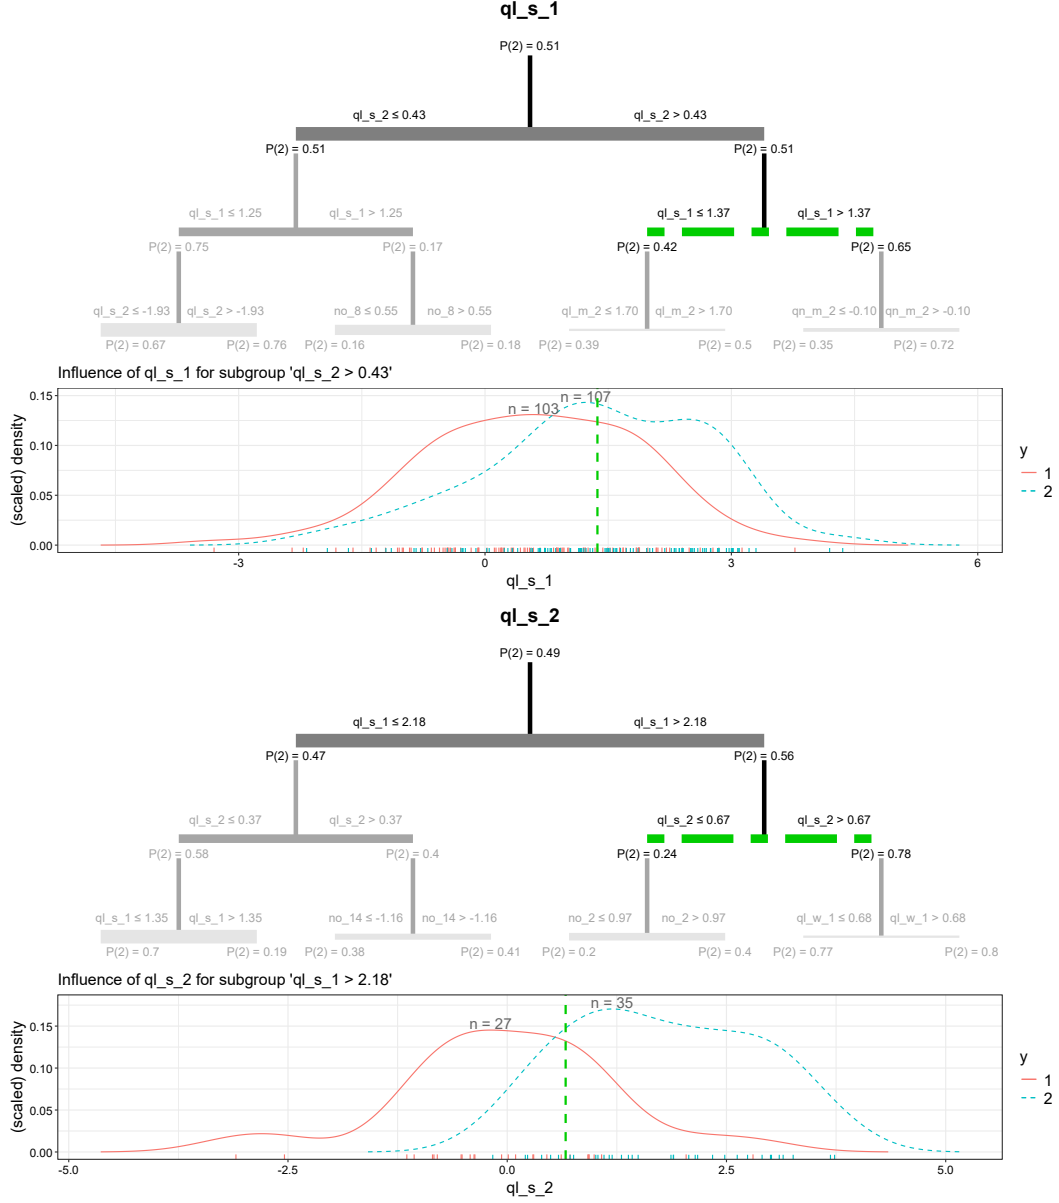

Fig. S12: Visualization of the CRTRs for the covariates  $X_{ql\_s\_1}$  and  $X_{ql\_s\_2}$  in a dataset generated from DGP 1 ( $n = 500$ ). The thickness of the horizontal lines reflects the covariate scores, dashed lines indicate top-scoring splits, and gray-shaded areas mark tree regions outside these splits and their ancestors. The class frequency distributions at the nodes and the weighted kernel density estimates of the class-specific covariate distributions were computed using the in-bag data.  $P(2)$  denotes the in-bag proportion of observations belonging to class 2 at the respective node. Covariate labels are abbreviated (e.g.,  $ql\_s\_1$  denotes  $X_{ql\_s\_1}$  and  $no\_*$  denotes non-informative covariates)

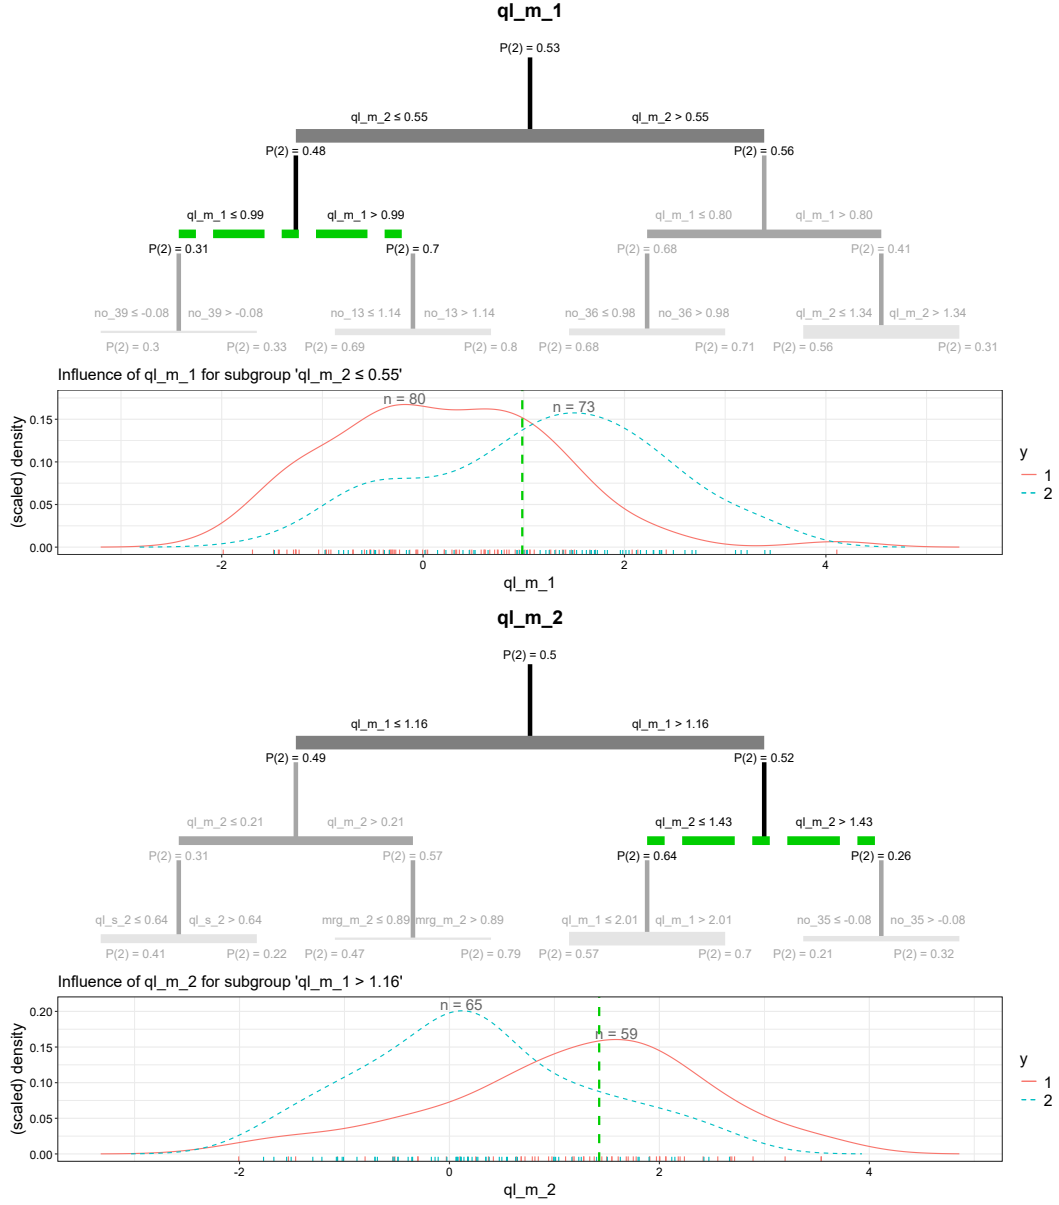

Fig. S13: Visualization of the CRTRs for the covariates  $X_{ql.m.1}$  and  $X_{ql.m.2}$  in a dataset generated from DGP 1 ( $n = 500$ ). The thickness of the horizontal lines reflects the covariate scores, dashed lines indicate top-scoring splits, and gray-shaded areas mark tree regions outside these splits and their ancestors. The class frequency distributions at the nodes and the weighted kernel density estimates of the class-specific covariate distributions were computed using the in-bag data.  $P(2)$  denotes the in-bag proportion of observations belonging to class 2 at the respective node. Covariate labels are abbreviated (e.g.,  $ql.m.1$  denotes  $X_{ql.m.1}$  and  $no_*$  denotes non-informative covariates)

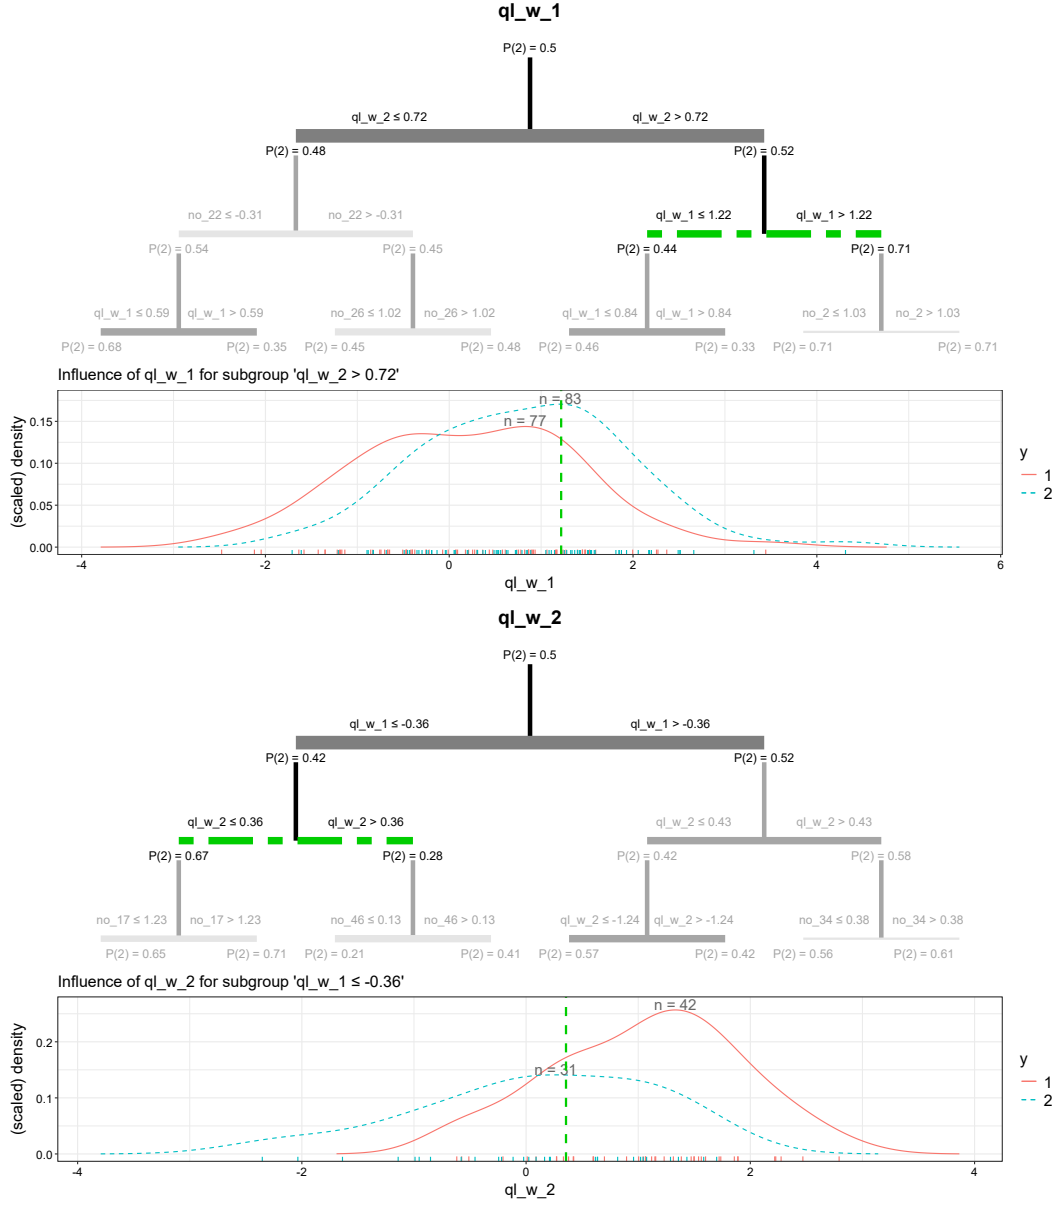

Fig. S14: Visualization of the CRTRs for the covariates  $X_{ql\_w\_1}$  and  $X_{ql\_w\_2}$  in a dataset generated from DGP 1 ( $n = 500$ ). The thickness of the horizontal lines reflects the covariate scores, dashed lines indicate top-scoring splits, and gray-shaded areas mark tree regions outside these splits and their ancestors. The class frequency distributions at the nodes and the weighted kernel density estimates of the class-specific covariate distributions were computed using the in-bag data.  $P(2)$  denotes the in-bag proportion of observations belonging to class 2 at the respective node. Covariate labels are abbreviated (e.g.,  $ql\_w\_1$  denotes  $X_{ql\_w\_1}$  and  $no\_*$  denotes non-informative covariates)

## D.2.2 DGP 2

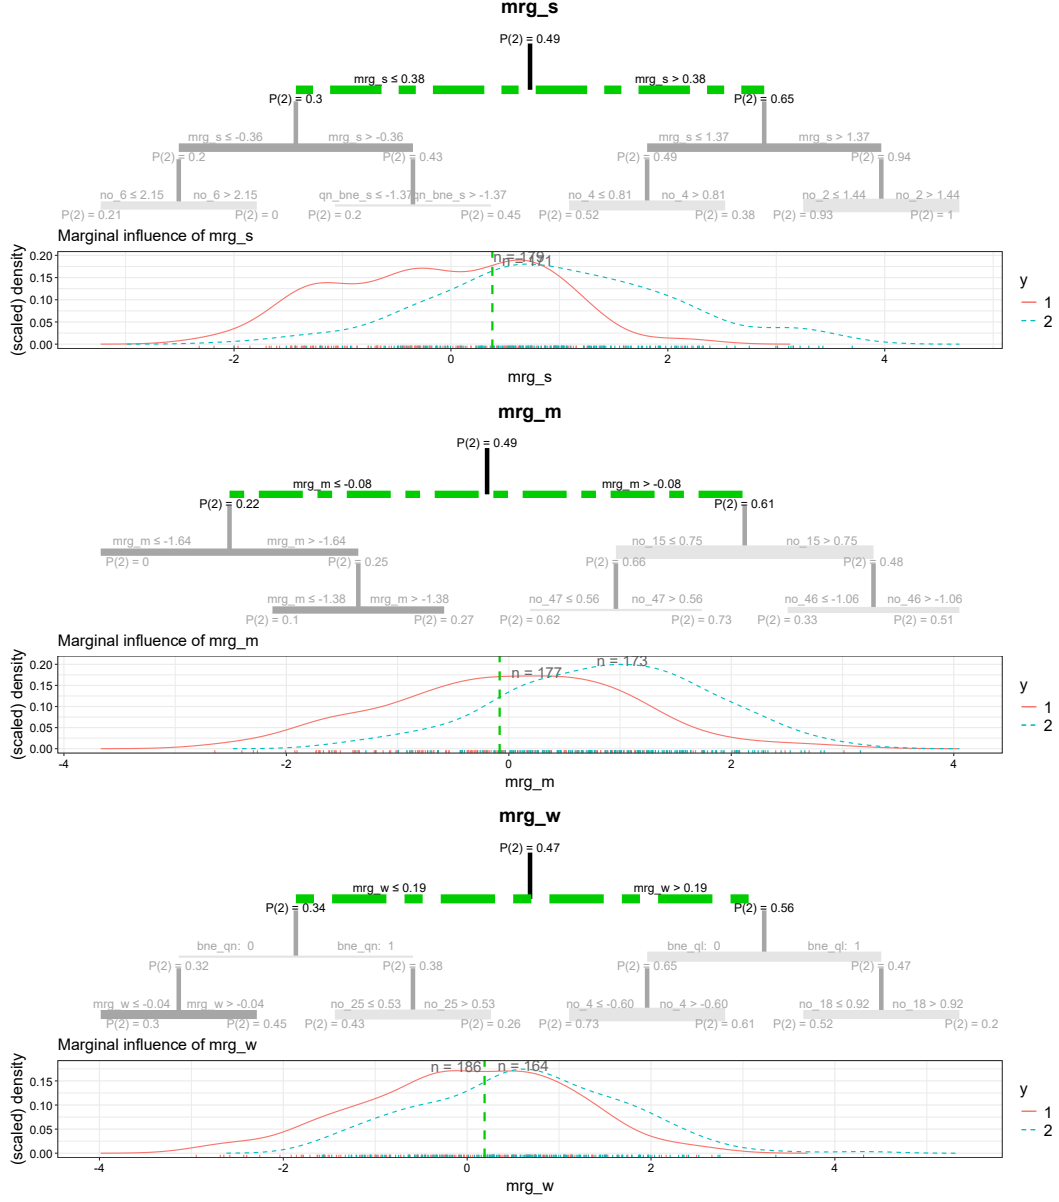

Fig. S15: Visualization of the CRTRs for the covariates  $X_{mrg\_s}$ ,  $X_{mrg\_m}$ , and  $X_{mrg\_w}$  in a dataset generated from DGP 2 ( $n = 500$ ). The thickness of the horizontal lines reflects the covariate scores, dashed lines indicate top-scoring splits, and gray-shaded areas mark tree regions outside these splits and their ancestors. The class frequency distributions at the nodes and the weighted kernel density estimates of the class-specific covariate distributions were computed using the in-bag data.  $P(2)$  denotes the in-bag proportion of observations belonging to class 2 at the respective node. Covariate labels are abbreviated (e.g.,  $mrg\_s$  denotes  $X_{mrg\_s}$  and  $no\_*$  denotes non-informative covariates)

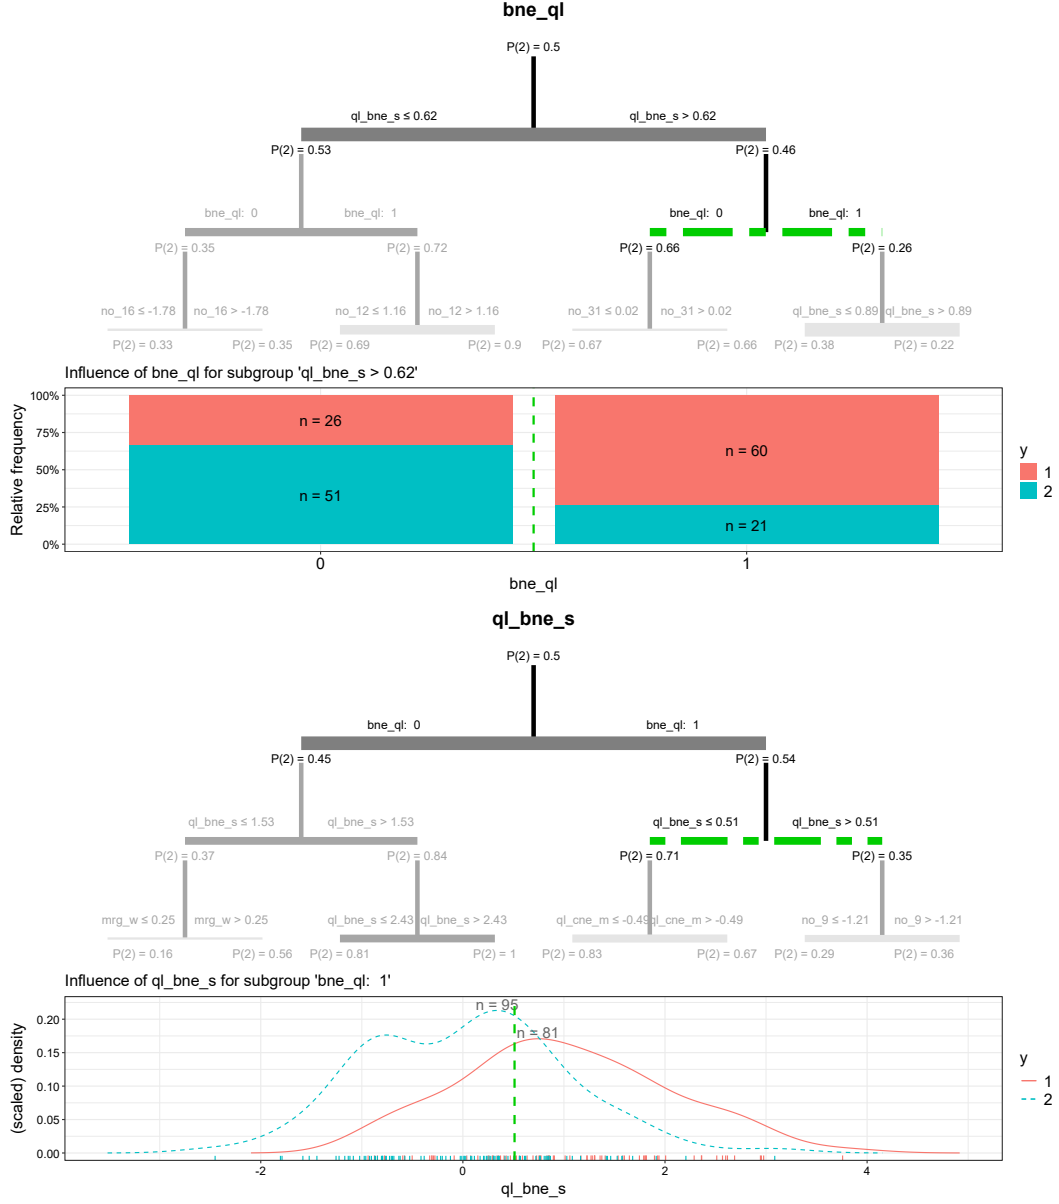

Fig. S16: Visualization of the CRTRs for the covariates  $X_{bne\_ql}$  and  $X_{ql\_bne\_s}$  in a dataset generated from DGP 2 ( $n = 500$ ). The thickness of the horizontal lines reflects the covariate scores, dashed lines indicate top-scoring splits, and gray-shaded areas mark tree regions outside these splits and their ancestors. The class frequency distributions at the nodes, the bar plots, and the weighted kernel density estimates of the class-specific covariate distributions were computed using the in-bag data.  $P(2)$  denotes the in-bag proportion of observations belonging to class 2 at the respective node. Covariate labels are abbreviated (e.g., **bne\_ql** denotes  $X_{bne\_ql}$  and **no\_\*** denotes non-informative covariates)

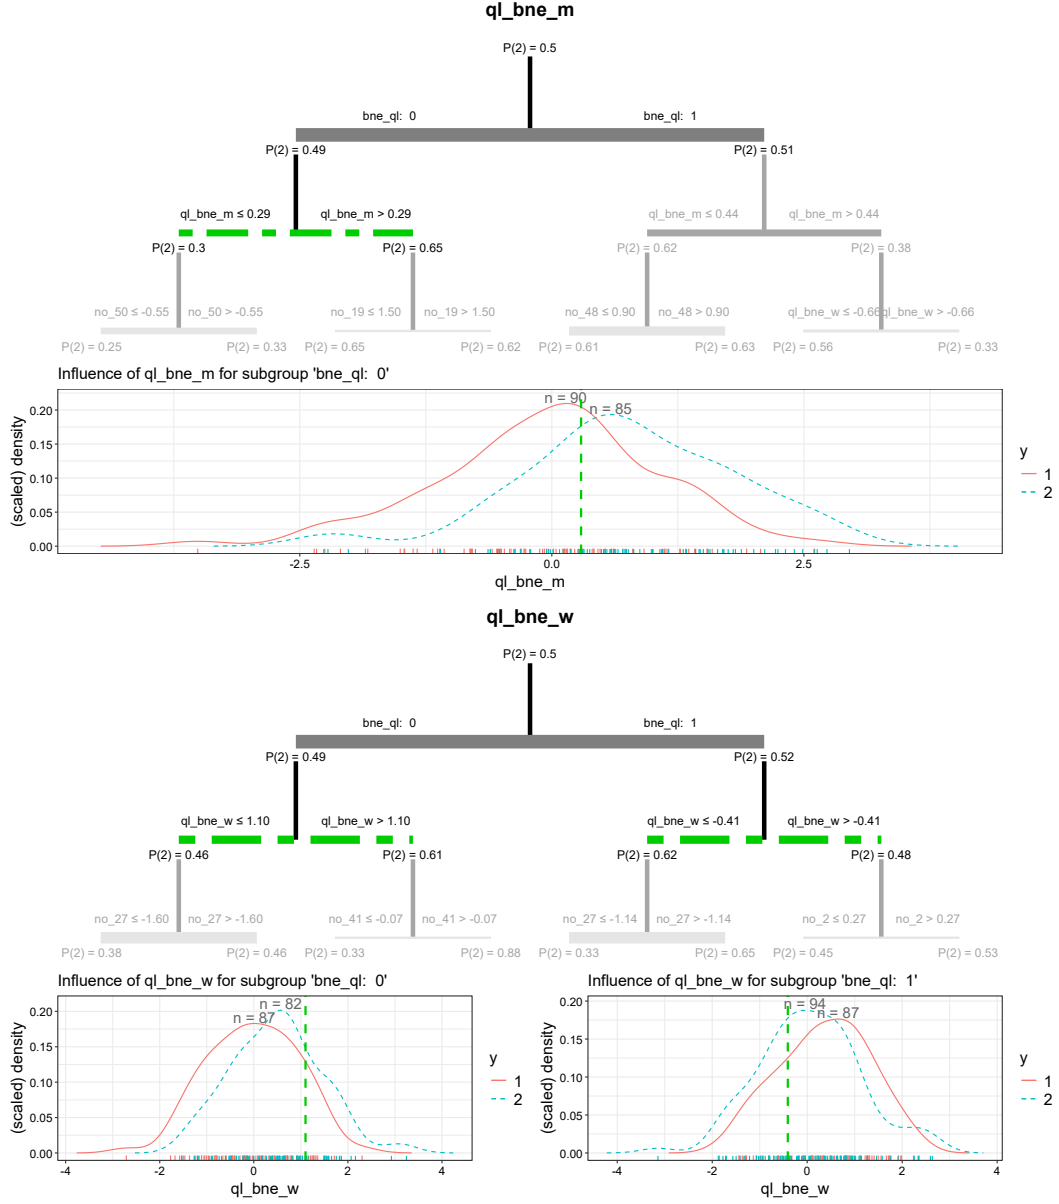

Fig. S17: Visualization of the CRTRs for the covariates  $X_{ql.bne.m}$  and  $X_{ql.bne.w}$  in a dataset generated from DGP 2 ( $n = 500$ ). The thickness of the horizontal lines reflects the covariate scores, dashed lines indicate top-scoring splits, and gray-shaded areas mark tree regions outside these splits and their ancestors. The class frequency distributions at the nodes and the weighted kernel density estimates of the class-specific covariate distributions were computed using the in-bag data.  $P(2)$  denotes the in-bag proportion of observations belonging to class 2 at the respective node. Covariate labels are abbreviated (e.g.,  $ql.bne.m$  denotes  $X_{ql.bne.m}$  and  $no.*$  denotes non-informative covariates)

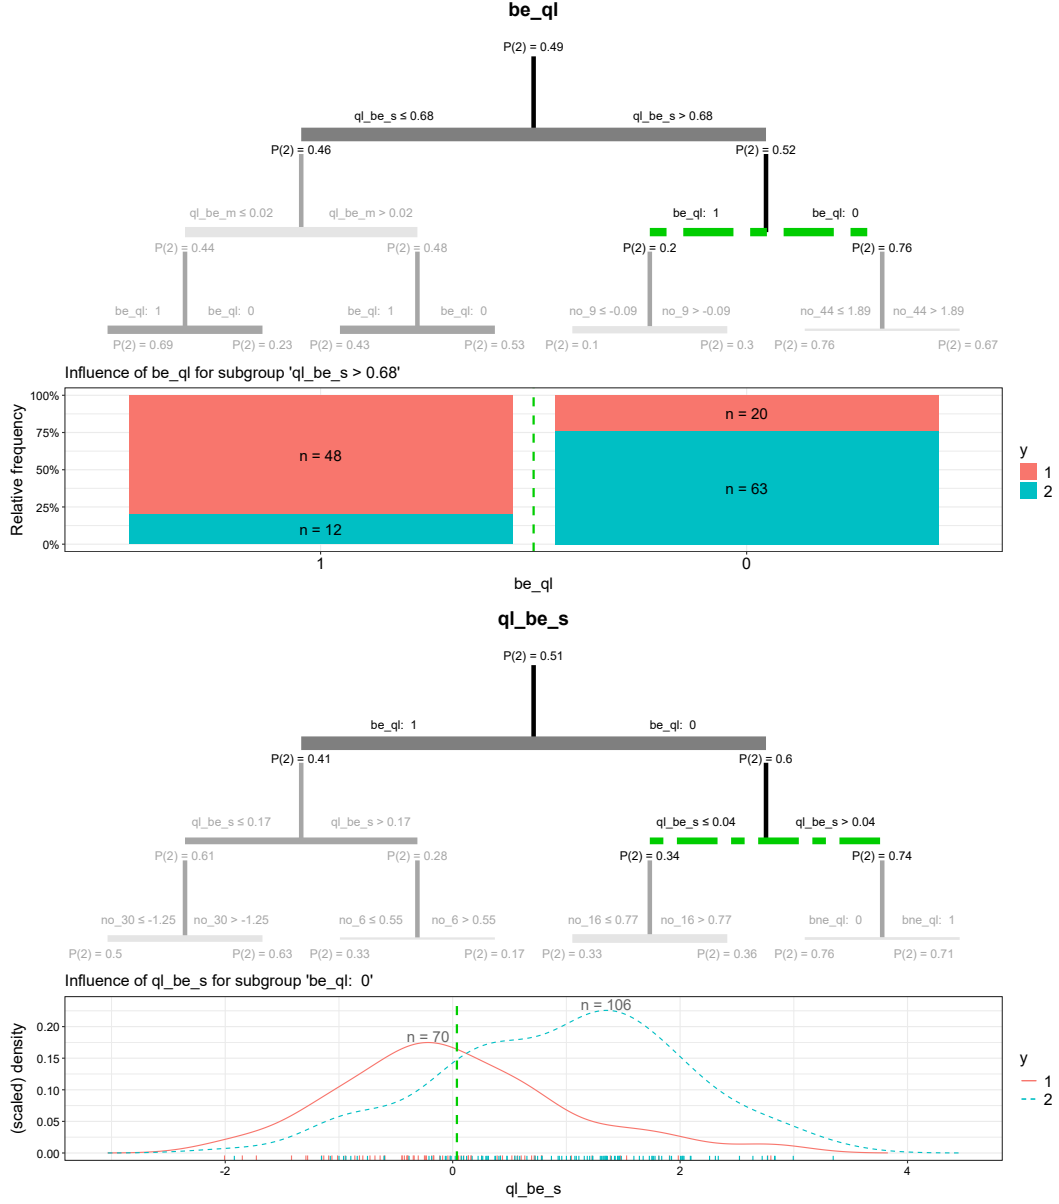

Fig. S18: Visualization of the CRTRs for the covariates  $X_{be\_ql}$  and  $X_{ql\_be\_s}$  in a dataset generated from DGP 2 ( $n = 500$ ). The thickness of the horizontal lines reflects the covariate scores, dashed lines indicate top-scoring splits, and gray-shaded areas mark tree regions outside these splits and their ancestors. The class frequency distributions at the nodes, the bar plots, and the weighted kernel density estimates of the class-specific covariate distributions were computed using the in-bag data.  $P(2)$  denotes the in-bag proportion of observations belonging to class 2 at the respective node. Covariate labels are abbreviated (e.g., **be\_ql** denotes  $X_{be\_ql}$  and **no\_\*** denotes non-informative covariates)

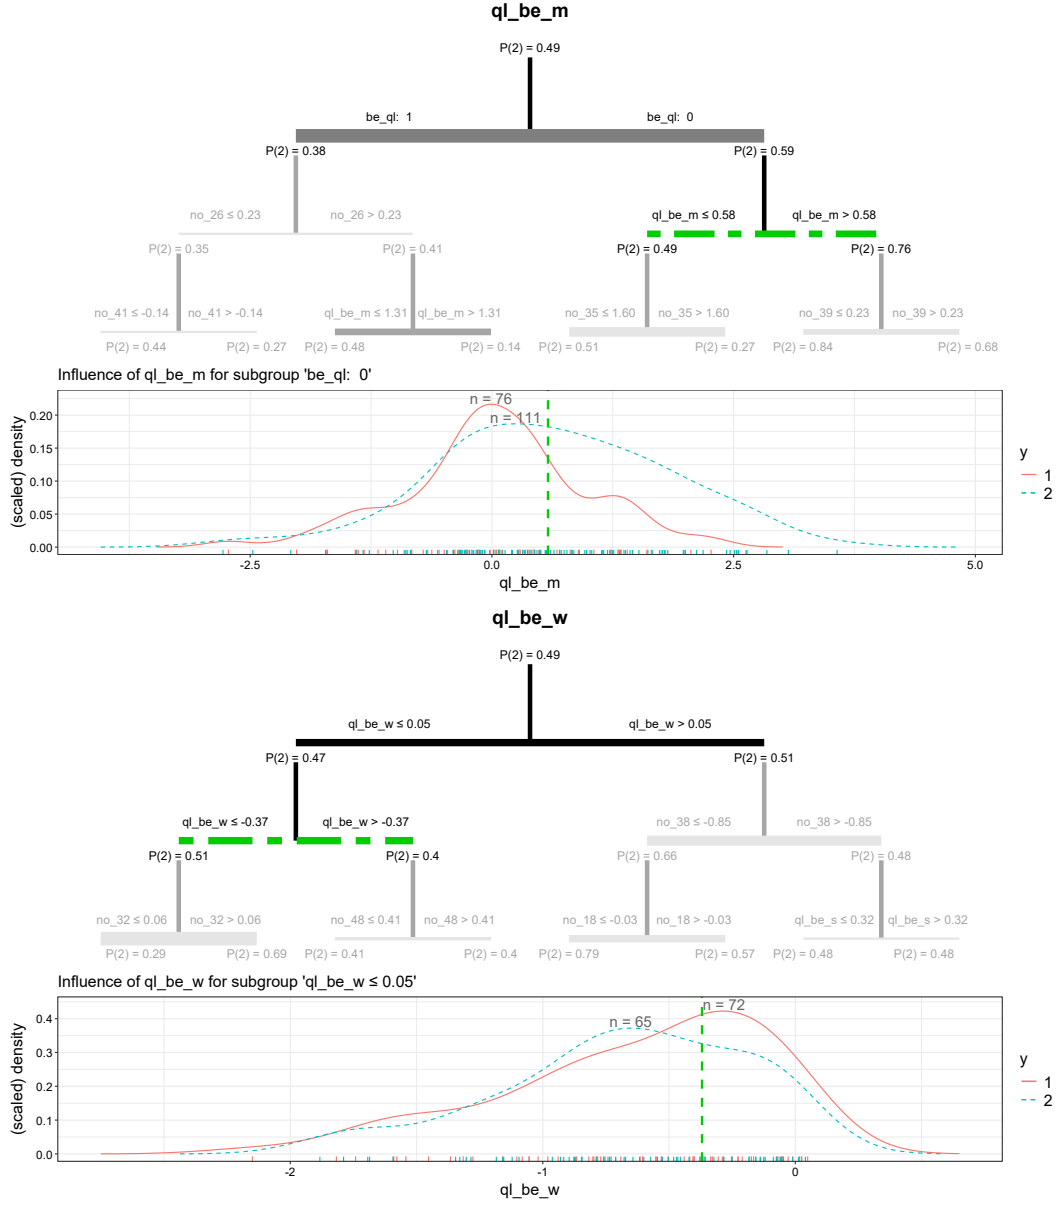

Fig. S19: Visualization of the CRTRs for the covariates  $X_{ql\_be\_m}$  and  $X_{ql\_be\_w}$  in a dataset generated from DGP 2 ( $n = 500$ ). The thickness of the horizontal lines reflects the covariate scores, dashed lines indicate top-scoring splits, and gray-shaded areas mark tree regions outside these splits and their ancestors. The class frequency distributions at the nodes and the weighted kernel density estimates of the class-specific covariate distributions were computed using the in-bag data.  $P(2)$  denotes the in-bag proportion of observations belonging to class 2 at the respective node. Covariate labels are abbreviated (e.g.,  $ql\_be\_m$  denotes  $X_{ql\_be\_m}$  and  $no\_*$  denotes non-informative covariates)

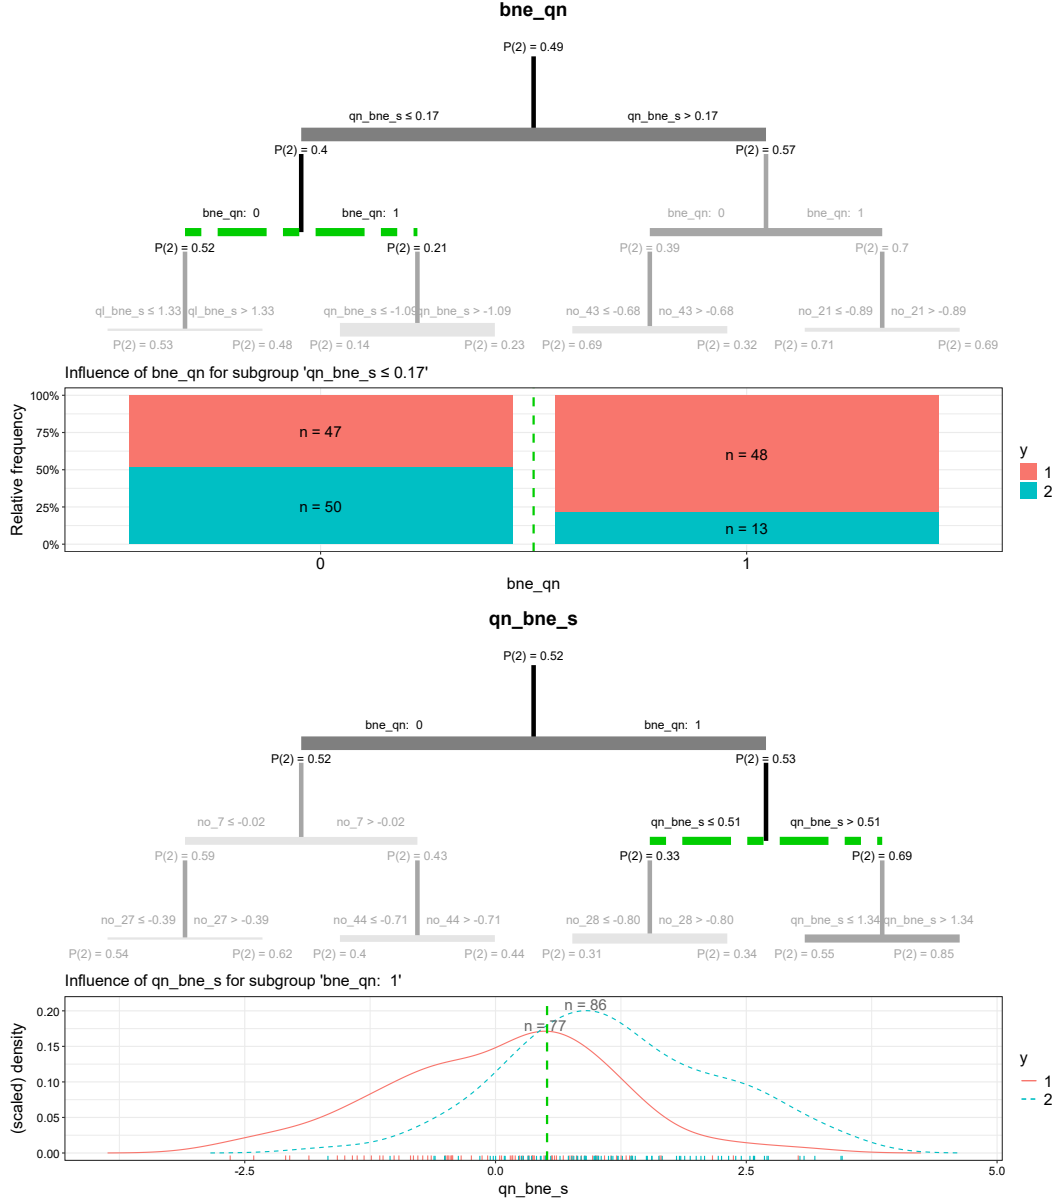

Fig. S20: Visualization of the CRTRs for the covariates  $X_{bne\_qn}$  and  $X_{qn\_bne\_s}$  in a dataset generated from DGP 2 ( $n = 500$ ). The thickness of the horizontal lines reflects the covariate scores, dashed lines indicate top-scoring splits, and gray-shaded areas mark tree regions outside these splits and their ancestors. The class frequency distributions at the nodes, the bar plots, and the weighted kernel density estimates of the class-specific covariate distributions were computed using the in-bag data.  $P(2)$  denotes the in-bag proportion of observations belonging to class 2 at the respective node. Covariate labels are abbreviated (e.g., **bne\_qn** denotes  $X_{bne\_qn}$  and **no\_\*** denotes non-informative covariates)

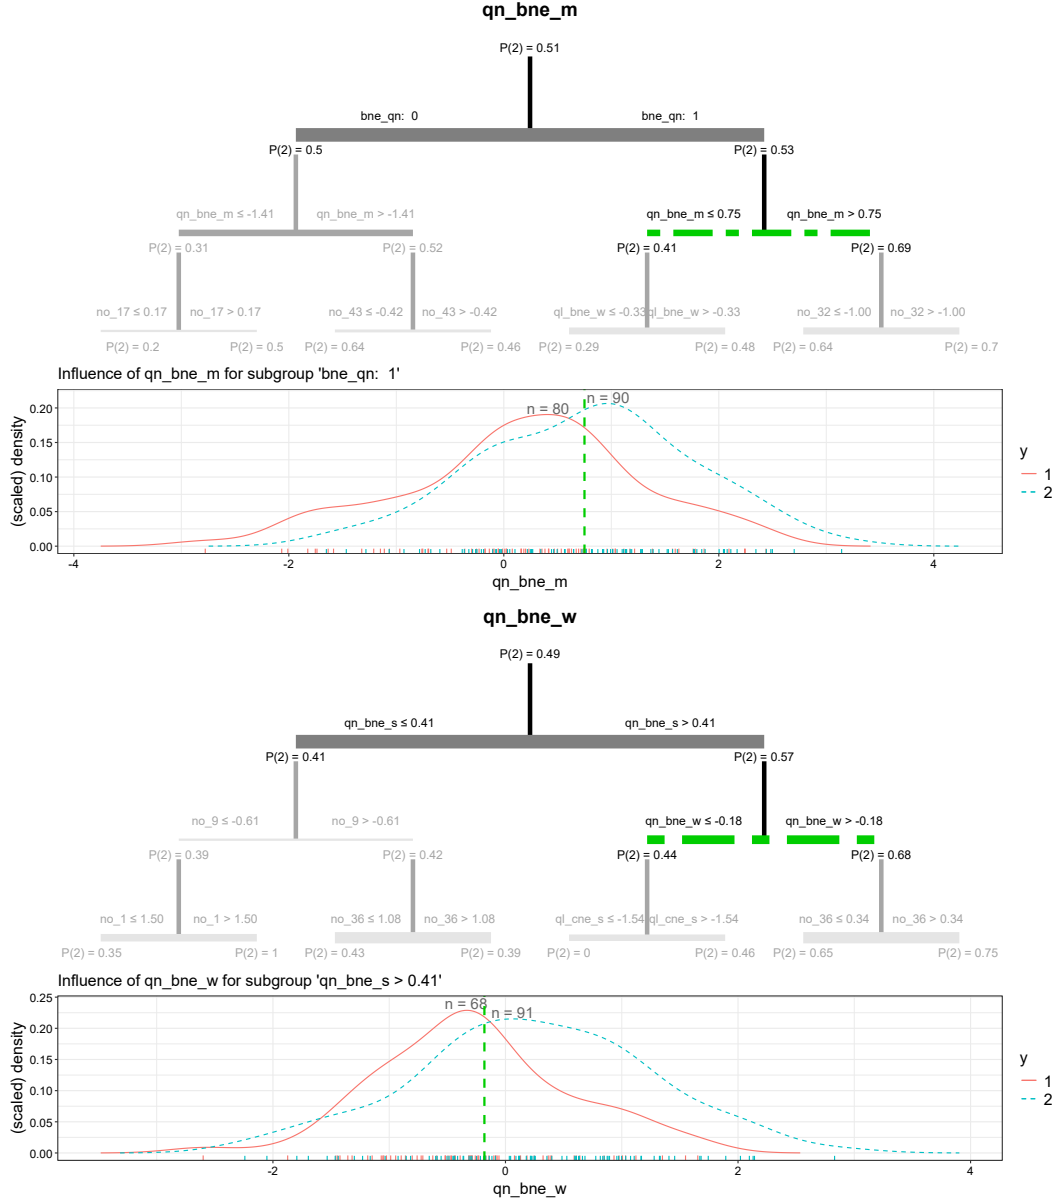

Fig. S21: Visualization of the CRTRs for the covariates  $X_{qn.be.m}$  and  $X_{qn.be.w}$  in a dataset generated from DGP 2 ( $n = 500$ ). The thickness of the horizontal lines reflects the covariate scores, dashed lines indicate top-scoring splits, and gray-shaded areas mark tree regions outside these splits and their ancestors. The class frequency distributions at the nodes and the weighted kernel density estimates of the class-specific covariate distributions were computed using the in-bag data.  $P(2)$  denotes the in-bag proportion of observations belonging to class 2 at the respective node. Covariate labels are abbreviated (e.g.,  $qn.be.m$  denotes  $X_{qn.be.m}$  and  $no.*$  denotes non-informative covariates)

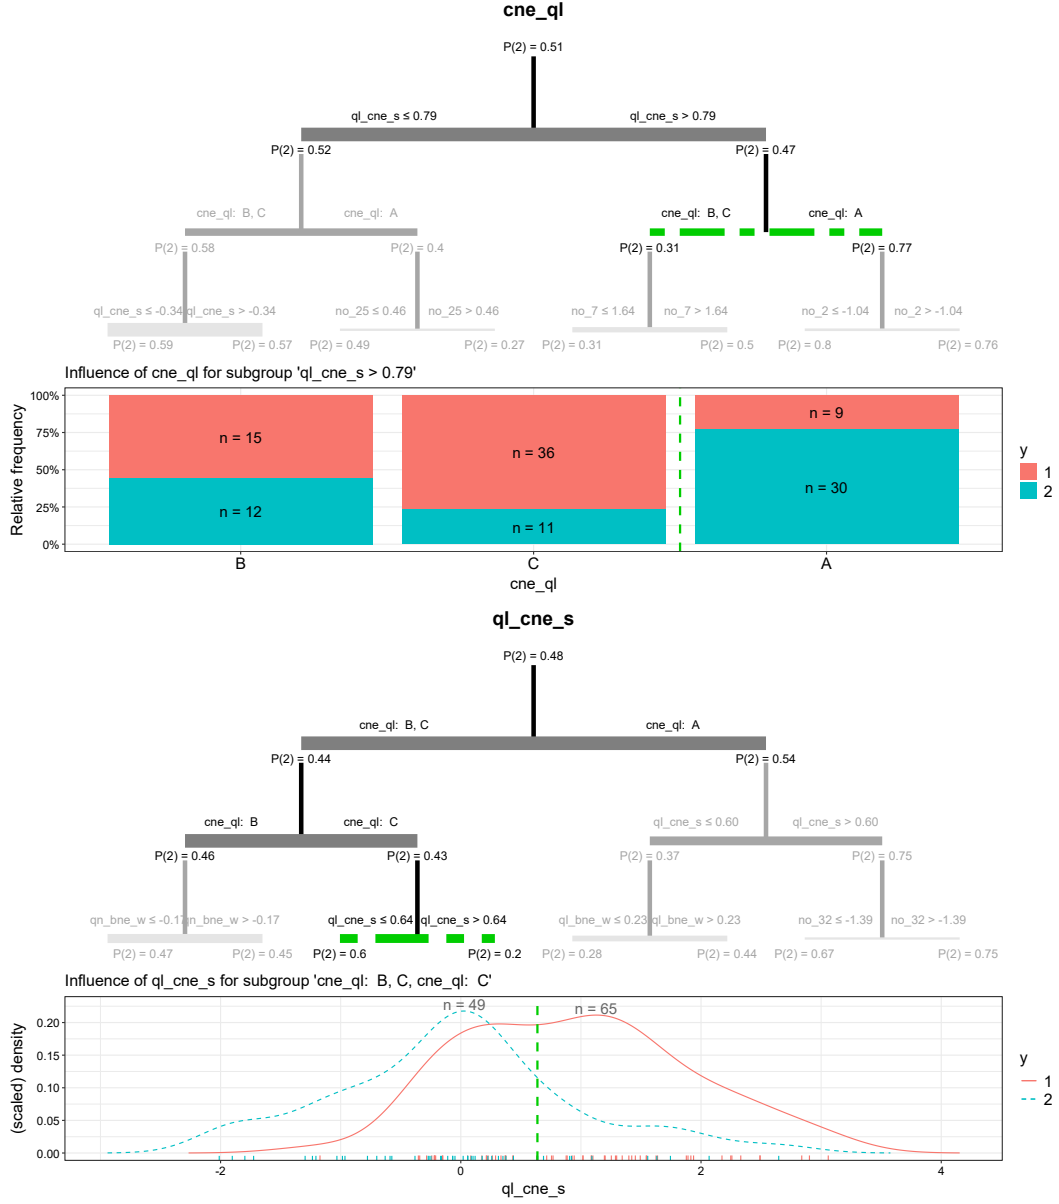

Fig. S22: Visualization of the CRTRs for the covariates  $X_{cne\_ql}$  and  $X_{ql\_cne\_s}$  in a dataset generated from DGP 2 ( $n = 500$ ). The thickness of the horizontal lines reflects the covariate scores, dashed lines indicate top-scoring splits, and gray-shaded areas mark tree regions outside these splits and their ancestors. The class frequency distributions at the nodes, the bar plots, and the weighted kernel density estimates of the class-specific covariate distributions were computed using the in-bag data.  $P(2)$  denotes the in-bag proportion of observations belonging to class 2 at the respective node. Covariate labels are abbreviated (e.g., **cne\_ql** denotes  $X_{cne\_ql}$  and **no\_\*** denotes non-informative covariates)

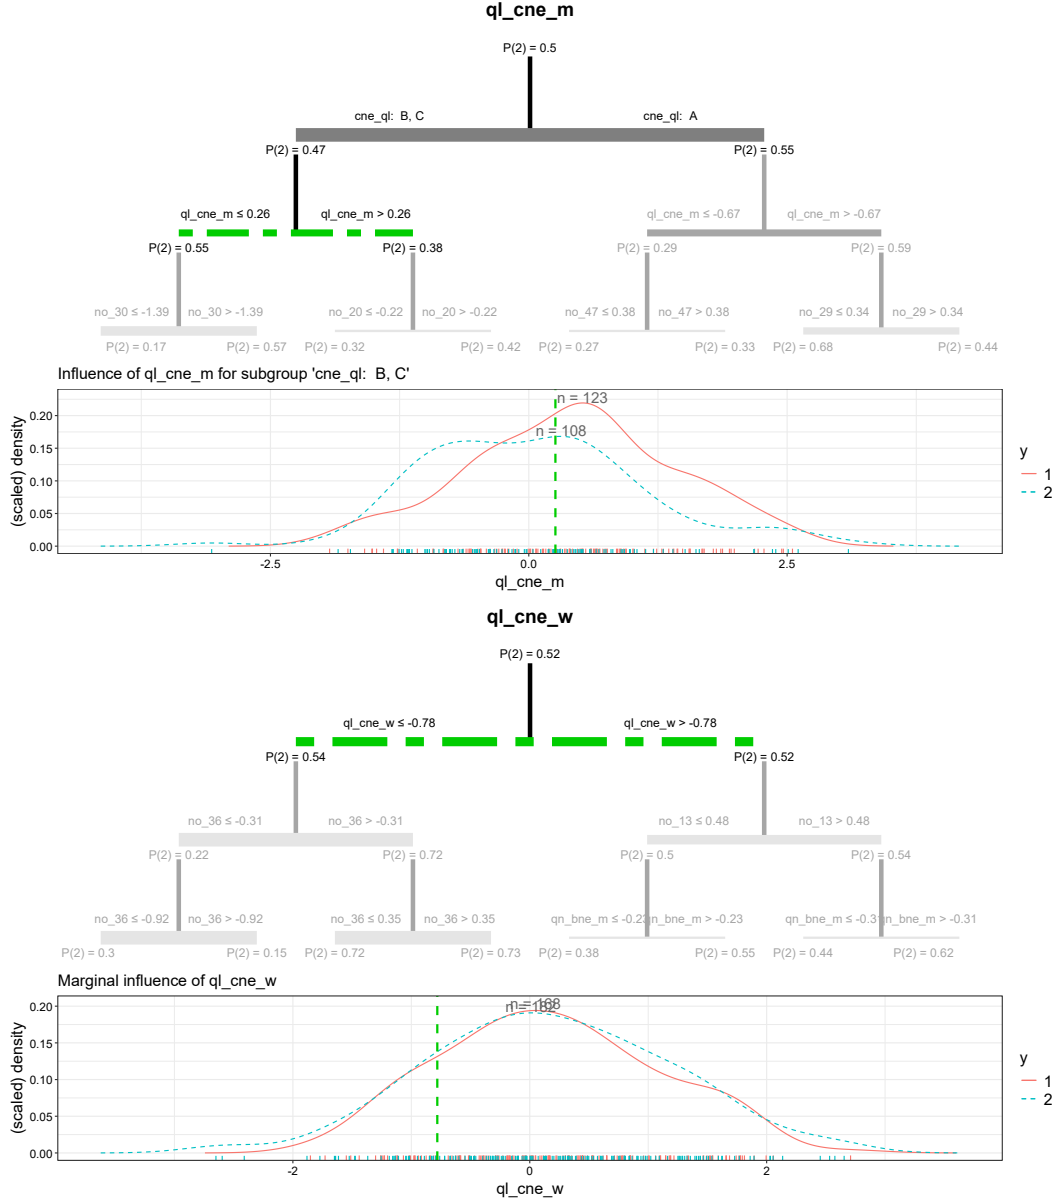

Fig. S23: Visualization of the CRTRs for the covariates  $X_{ql\_cne\_m}$  and  $X_{ql\_cne\_w}$  in a dataset generated from DGP 2 ( $n = 500$ ). The thickness of the horizontal lines reflects the covariate scores, dashed lines indicate top-scoring splits, and gray-shaded areas mark tree regions outside these splits and their ancestors. The class frequency distributions at the nodes and the weighted kernel density estimates of the class-specific covariate distributions were computed using the in-bag data.  $P(2)$  denotes the in-bag proportion of observations belonging to class 2 at the respective node. Covariate labels are abbreviated (e.g.,  $ql\_cne\_m$  denotes  $X_{ql\_cne\_m}$  and  $no\_*$  denotes non-informative covariates)

### D.3 Wine Dataset: Unity VIM and Permutation VIM Values

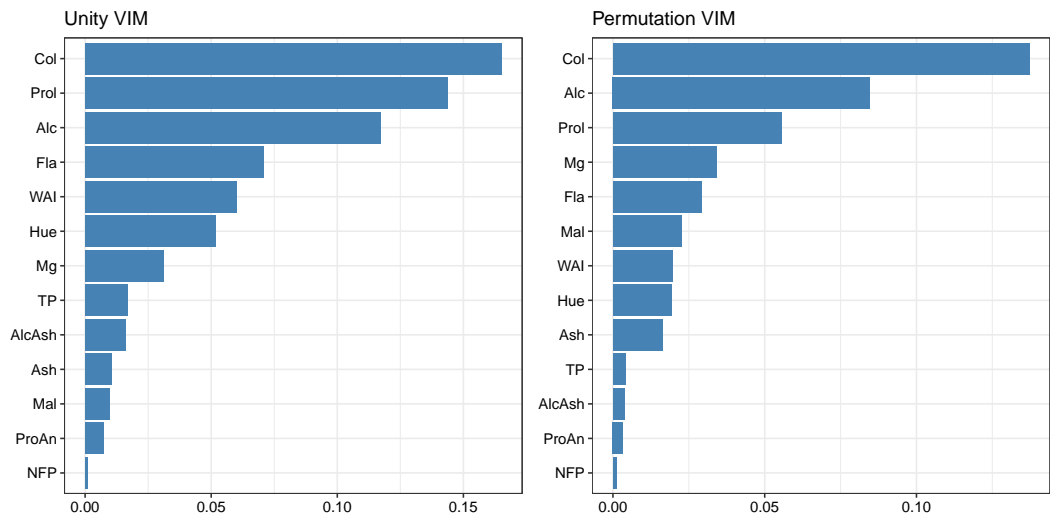

Fig. S24: Unity and permutation VIM values for wine dataset ( $n = 178$ )

## References

- Don Coppersmith, Se June Hong, and Jonathan RM Hosking. Partitioning nominal attributes in decision trees. *Data Mining and Knowledge Discovery*, 3:197–217, 1999. doi:10.1023/A:1009869804967.
- Roman Hornung and Anne-Laure Boulesteix. Interaction forests: Identifying and exploiting interpretable quantitative and qualitative interaction effects. *Computational Statistics & Data Analysis*, 171:107460, 2022. doi:10.1016/j.csda.2022.107460.
- Silke Janitza, Carolin Strobl, and Anne-Laure Boulesteix. An AUC-based permutation variable importance measure for random forests. *BMC Bioinformatics*, 14:119, 2013. doi:10.1186/1471-2105-14-119.
- Xiao Li, Yu Wang, Sumanta Basu, Karl Kumbier, and Bin Yu. A debiased MDI feature importance measure for random forests. *Advances in Neural Information Processing Systems*, 32:1–17, 2019.
- Markus Loecher. Unbiased variable importance for random forests. *Communications in Statistics - Theory and Methods*, 51(5):1413–1425, 2020. doi:10.1080/03610926.2020.1764042.
- Massimiliano Pastore and Antonio Calcagni. Measuring distribution similarities between samples: a distribution-free overlapping index. *Frontiers in Psychology*, 10:1089, 2019. doi:10.3389/fpsyg.2019.01089.
- Philipp Probst, Anne-Laure Boulesteix, and Bernd Bischl. Tunability: Importance of hyperparameters of machine learning algorithms. *Journal of Machine Learning Research*, 20:1–32, 2019.
- Zhengze Zhou and Giles Hooker. Unbiased measurement of feature importance in tree-based methods. *ACM Transactions on Knowledge Discovery from Data*, 15(2):1–21, 2021. doi:10.1145/3429445.
